# Supplementary material for: Bootstrap Embedding on a Quantum Computer
Source: arXiv:2301.01457 ancillary file (2023-04-25)
Supplement: Supplementary file 1 [file SI.pdf]

# Supporting Information for “Bootstrap Embedding on a Quantum Computer”

Yuan Liu,<sup>1,\*</sup> Oinam R. Meitei,<sup>2</sup> Zachary E. Chin,<sup>1</sup> Arkopal  
Dutt,<sup>3</sup> Max Tao,<sup>4</sup> Isaac L. Chuang,<sup>1,5</sup> and Troy Van Voorhis<sup>2,†</sup>

<sup>1</sup>*Department of Physics, Co-Design Center for Quantum Advantage,  
Massachusetts Institute of Technology, Cambridge, Massachusetts 02139, USA*

<sup>2</sup>*Department of Chemistry, Massachusetts Institute of Technology, Cambridge, Massachusetts 02139, USA*

<sup>3</sup>*Department of Mechanical Engineering, Massachusetts Institute of Technology, Cambridge, Massachusetts 02139, USA*

<sup>4</sup>*Department of Physics, Massachusetts Institute of Technology, Cambridge, Massachusetts 02139, USA*

<sup>5</sup>*Department of Electrical Engineering and Computer Science,  
Massachusetts Institute of Technology, Cambridge, Massachusetts 02139, USA*

(Dated: April 25, 2023)

## CONTENTS

|                                                                                 |    |
|---------------------------------------------------------------------------------|----|
| S1. Construction of the Embedding Hamiltonians                                  | 2  |
| S2. Basis Transformation Unitary from Localized to Canonical Molecular Orbitals | 2  |
| S3. Proof of Equivalence of the Linear and Quadratic Constraint                 | 3  |
| S4. Estimating Quadratic Penalty from Subsystem SWAP Test                       | 4  |
| A. Quantum Circuit of the SWAP Test                                             | 4  |
| B. Ancilla Measurement Probability                                              | 4  |
| C. Connection to Quadratic Penalty                                              | 6  |
| S5. Eigenvalue Equations for the Quadratic Penalty Method                       | 6  |
| A. Derivative $\frac{\partial \mathcal{L}_A}{\partial C_{ai\mu}}$               | 7  |
| B. Derivative $\frac{\partial C_{ai\mu}}{\partial V_{BE}}$                      | 8  |
| C. Gradient of Cost Function versus BE Potential                                | 10 |
| S6. Sample Complexity for Estimating the Overlap from Tomography                | 10 |
| S7. Details of Quantum Amplitude Estimation and Quadratic Speedup               | 12 |
| A. Amplitude Amplification                                                      | 12 |
| B. Estimate the Amplitude from Binary Search                                    | 14 |
| C. Quadratic Speedup                                                            | 15 |
| S8. QBE Algorithm Using Naive RDM Linear Matching                               | 16 |
| S9. Computational Details                                                       | 17 |
| A. FCI and QPE Eigensolver Runtime Benchmark                                    | 17 |
| B. Classical Bootstrap Embedding with VMC and FCI as Eigensolver                | 17 |
| C. SWAP Test Circuit in Quantum Bootstrap Embedding                             | 18 |
| D. Quantum Bootstrap Embedding Calculation                                      | 18 |
| 1. QBE Iterations                                                               | 18 |
| 2. Calculation of Total System Energy                                           | 18 |
| E. Details of VQE Eigensolver                                                   | 21 |
| References                                                                      | 23 |

---

\* yuanliu@mit.edu

† tvan@mit.edu

## S1. CONSTRUCTION OF THE EMBEDDING HAMILTONIANS

The one- and two-electron integrals  $h_{pq}^{(A)}$  and  $V_{pqrs}^{(A)}$  of the embedding Hamiltonian for a chosen fragment  $A$  in Eq. (5) of the main text can be obtained from transforming the original integrals of the total system by a projector  $T^{(A)}$

$$\begin{aligned} h_{pq}^{(A)} &= \sum_{\mu\nu}^N T_{\mu p}^{(A)} F_{\mu\nu}^{(\text{env}, A)} T_{\nu q}^{(A)} \\ V_{pqrs}^{(A)} &= \sum_{\mu\nu\lambda\sigma}^N T_{\mu p}^{(A)} T_{\nu q}^{(A)} V_{\mu\nu\lambda\sigma} T_{\lambda r}^{(A)} T_{\sigma s}^{(A)}, \end{aligned} \quad (\text{S1})$$

where  $F^{(\text{env}, A)}$  is the Fock matrix of the environment and  $T^{(A)}$  is a projection matrix that transform the one- and two-electron integrals in Eq. (1) to the EO basis. In practice,  $T^{(A)}$  can be obtained by performing an SVD of the off-diagonal Hartree-Fock density matrix  $P_{\mu\nu}^{(A)}$ ,

$$P_{\mu\nu}^{(A)} = U_A \Sigma_A V_A^\dagger \quad (\text{S2})$$

$$T^{(A)} = \left[ \begin{array}{c|c} I & \\ \hline & U_A \end{array} \right]. \quad (\text{S3})$$

The integral transformations in Eq. (S1) can be performed efficiently on classical computers.

## S2. BASIS TRANSFORMATION UNITARY FROM LOCALIZED TO CANONICAL MOLECULAR ORBITALS

Bootstrap embedding requires *spatially* local information on overlapping sites of a quantum system to match, whereas this local basis may not be the same as the most convenient computational basis. For example, many state preparation ansatz on a quantum computer is designed to work the best under the canonical molecular orbitals (delocalized, obtained from a Hartree-Fock calculation) as the computational basis, where a basis transformation to local atomic basis are required afterwards to extract spatially local information. In this section, we give a unitary that can achieve such a basis transformation from MOs to LOs on a quantum computer, from an early result due to Thouless [1] which is also employed in a recent work [2].

Given two set of single-particle orbitals,  $\{\psi_p\}$  and  $\{\phi_q\}$  to represent the MOs and the LOs, respectively. Furthermore, denote the basis rotation between the two as

$$\phi_p = \sum_{q=1}^n [e^{ih}]_{pq} \psi_q \quad (\text{S4})$$

where  $h$  is an  $n \times n$  hermitian matrix,  $[e^{ih}]_{pq}$  is the  $(p, q)$ -th element of the orbital rotation unitary. For notation purpose, we also associate each MO  $\psi_q$  with a creation and annihilation operator  $a_p^\dagger, a_p$ .

This orbital rotation from the MOs to the LOs will induce a unitary transformation on the Slater determinants written under these two set of orbitals. More concretely, suppose  $|\Psi\rangle$  and  $|\Phi\rangle$  are representation of the same mean-field state using orbitals  $\{\psi_p\}$  and  $\{\phi_q\}$ , respectively, then it can be shown [1] that the transformation between  $|\Psi\rangle$  and  $|\Phi\rangle$  is essentially a unitary operator generated by a 1-body operator in the MO basis

$$|\Phi\rangle = U_h |\Psi\rangle \quad (\text{S5})$$

where

$$U_h = e^{i \sum_{p,q=1}^n h_{pq} a_p^\dagger a_q}. \quad (\text{S6})$$

The above results on the transformation between two Slater determinants can be easily generalized to two arbitrary many-body quantum states  $|\Phi\rangle$  and  $|\Psi\rangle$  that represent the same underlying quantum state using the two different orbital sets, as we will show in the following. We can always write  $|\Phi\rangle$  as a linear combination of many Slater

determinants constructed from the orbital set  $\{\phi_p\}$

$$|\Phi\rangle = \sum_{\alpha} C_{\alpha} |\Phi_{\alpha}\rangle. \quad (\text{S7})$$

Using the unitary transformation  $U_h$  for each Slater determinant in  $|\Phi\rangle$ , we have

$$|\Phi\rangle = \sum_{\alpha} C_{\alpha} |\Phi_{\alpha}\rangle = \sum_{\alpha} C_{\alpha} U_h |\Psi_{\alpha}\rangle = U_h |\Psi\rangle, \quad (\text{S8})$$

where we have defined a new many-body state  $|\Psi\rangle$  using the same many-body coefficients  $C_{\alpha}$  but with the old MO Slater determinants  $|\Psi_{\alpha}\rangle$ . Equivalently, this means the transformation of a many-body state under orbital rotations follows the same unitary  $U_h$ .

On a quantum computer, in the case of Jordan-Wigner mapping, there is a direct one-to-one correspondence between Slater determinants and qubit states. Therefore the unitary transformation on a quantum computer to transform a state from MO to LO representation is to write  $U_h$  in its Jordan-Wigner form using

$$a_p^{\dagger} = \sigma_p^{+} \otimes Z_{p-1}^{\rightarrow}, \quad a_q = \sigma_q^{-} \otimes Z_{q-1}^{\rightarrow}, \quad (\text{S9})$$

where

$$Z_j^{\rightarrow} = Z_j \otimes Z_{j-1} \otimes \cdots \otimes Z_1 \otimes Z_0. \quad (\text{S10})$$

Note that the hermitian matrix  $h$  can be obtained from standard quantum chemistry package such as PySCF [3].

### S3. PROOF OF EQUIVALENCE OF THE LINEAR AND QUADRATIC CONSTRAINT

In this section, we prove the equivalent of the linear and the quadratic constraints in Eqs. (16) and (20).

Recall that in the main text (Eq. (15)), in a general case of  $m$  overlapping qubits, the mixed state reduced density matrices  $\rho_R^{(A)}$  can be written as

$$\rho_R^{(A)} = \frac{I + \sum_{\alpha=1}^{4^m-1} \langle \Sigma_{\alpha} \rangle_A \Sigma_{\alpha}}{2^m}. \quad (\text{S11})$$

In the special case of  $m = 1$ , we recover the usual expression for a single-qubit density matrix.

The forward direction of deriving Eq. (20) from (16) is trivial, because if  $\langle \Sigma_{\alpha} \rangle_A = \langle \Sigma_{\alpha} \rangle_B$  for all  $\alpha$ , this means  $\rho_R^{(A)} = \rho_R^{(B)}$  which leads to Eq. (20).

Now we focus on showing the reverse is true by deriving Eq. (16) from (20). Substitute (S11) into (20), we obtain

$$\text{Tr}[(\rho_R^{(A)} - \rho_R^{(B)})^2] = \frac{1}{2^m} \sum_{\alpha, \beta=1}^{4^m-1} (\langle \Sigma_{\alpha} \rangle_A - \langle \Sigma_{\alpha} \rangle_B) (\langle \Sigma_{\beta} \rangle_A - \langle \Sigma_{\beta} \rangle_B) \text{Tr}[\Sigma_{\alpha} \Sigma_{\beta}]. \quad (\text{S12})$$

Choose a convenient basis for the Hermitian generators  $\Sigma_{\alpha}$  by express them as tensor product of  $m$  SU(2) Paulis  $\{\sigma_{\alpha_m}\}$

$$\Sigma_{\alpha} = \sigma_{\alpha_1} \otimes \sigma_{\alpha_2} \otimes \cdots \otimes \sigma_{\alpha_m}, \quad (\text{S13})$$

we immediately see that

$$\text{Tr}[\Sigma_{\alpha} \Sigma_{\beta}] = \text{Tr}[(\sigma_{\alpha_1} \sigma_{\beta_1}) \otimes (\sigma_{\alpha_2} \sigma_{\beta_2}) \otimes \cdots \otimes (\sigma_{\alpha_m} \sigma_{\beta_m})] \quad (\text{S14})$$

$$= \prod_{s=1}^m \text{Tr}[\sigma_{\alpha_s} \sigma_{\beta_s}] \quad (\text{S15})$$

$$= \prod_{s=1}^m (2\delta_{\alpha_s, \beta_s}) \quad (\text{S16})$$

$$= 2^m \delta_{\alpha\beta} \quad (\text{S17})$$

where we define a composite index (bold font)  $\alpha = (\alpha_1 \alpha_2 \cdots \alpha_k)$  and  $\beta = (\beta_1 \beta_2 \cdots \beta_k)$ . Substitute (S17) into (S12) and note that  $\delta_{\alpha\beta} = \delta_{\alpha\beta}$ , we obtain

$$\text{Tr}[(\rho_R^{(A)} - \rho_R^{(B)})^2] = \sum_{\alpha=1}^{4^m-1} (\langle \Sigma_\alpha \rangle_A - \langle \Sigma_\alpha \rangle_B)^2. \quad (\text{S18})$$

Given  $\langle \Sigma_\alpha \rangle$ 's as real numbers in usual implementation of electronic structure problems, then (S18) guarantees each individual term in the sum being zero, i.e.,

$$\langle \Sigma_\alpha \rangle_A - \langle \Sigma_\alpha \rangle_B = 0, \quad \forall i \in [1, 4^m - 1]. \quad (\text{S19})$$

This is equivalent to  $\rho_R^{(A)} = \rho_R^{(B)}$ . This completes the proof.  $\square$

#### S4. ESTIMATING QUADRATIC PENALTY FROM SUBSYSTEM SWAP TEST

In this section, we present details of the subsystem SWAP test and discuss how it can be used to estimate the quadratic penalty mismatch in (20) of the main text.

##### A. Quantum Circuit of the SWAP Test

The SWAP test as shown in Fig. 4 of the main text between two qubits can be directly generalized to a SWAP test between two quantum registers each of which contains multiple qubits. The idea is to use the upper ancilla qubit to perform multiple controlled-SWAP operations between all pairs of qubits in the two registers. For example, Fig. S5 performs a SWAP test between two pairs of qubits using a single ancilla qubit.

In our case, instead of performing SWAP test on the entire wave function of two fragments, we are interested to apply it to a subsystem of each fragment. In particular, denote qubits corresponding to the entire embedding orbitals as  $X_1 X_0$  for fragment  $X = A, B$ , where  $A_0$  and  $B_0$  are the subsystem on the overlapping region, whereas  $A_1$  and  $B_1$  are the rest of the embedding orbitals. Then a SWAP test between  $A_0$  and  $B_0$  can be performed in Fig. S1.

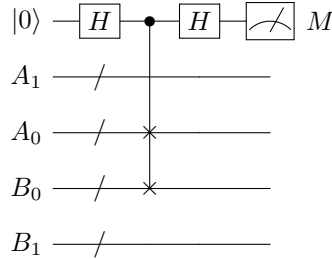

FIG. S1: Subsystem SWAP test between the overlapping regions of fragment  $A$  and  $B$ , where a controlled SWAP operation is performed on  $A_0$  and  $B_0$ . The measurement probability of the top ancilla qubit encodes information of the overlap.

##### B. Ancilla Measurement Probability

In the following, we show that the measurement probability of  $M$  in the upper ancilla qubit can be directly related to the overlap between the reduced density matrices on region  $A_0$  and  $B_0$ . This derivation can be performed in an arbitrary computational basis. For simplicity, we derive the results in the Schmidt basis of  $A_0$  and  $A_1$  (likewise for  $B$ ). Interest readers are encouraged to perform the derivation in an arbitrary basis as an exercise.

From Schmidt decomposition, the total wave function for fragment  $A$  and  $B$  can be written as

$$|\Psi_A\rangle = \sum_j a_j |A_{1,j}\rangle |A_{0,j}\rangle, \quad (\text{S20})$$

$$|\Psi_B\rangle = \sum_k b_k |B_{0,k}\rangle |B_{1,k}\rangle. \quad (\text{S21})$$

Denote the measurement outcome of the ancilla in Fig. S1 as  $M$ , it can be shown that

$$\text{Prob}[M = 0] = \frac{1}{2} [1 + \sum_{j,k} |a_j|^2 |b_k|^2 |\langle A_{0,j} | B_{0,k} \rangle|^2], \quad (\text{S22})$$

regardless of their environment  $A_1$  and  $B_1$ .

The above result can be understood as the overlap of the two reduced density matrix of fragments  $A$  and  $B$  in their overlapping region, as we can explicitly compute this in the following. From Eq. (S20) and (S21), the reduced density matrices of each is calculated to be

$$\begin{aligned} \rho_{A_0} &= \text{Tr}_{A_1} [|\Psi_A\rangle \langle \Psi_A|] \\ &= \text{Tr}_{A_1} \left[ \sum_{j,j'} a_j a_{j'}^* |A_{1,j}\rangle |A_{0,j}\rangle \langle A_{1,j'}| \langle A_{0,j'}| \right] \\ &= \sum_k \sum_{j,j'} a_j a_{j'}^* \langle A_{1,k} | A_{1,j}\rangle |A_{0,j}\rangle \langle A_{1,j'}| \langle A_{0,j'}| A_{1,k}\rangle \\ &= \sum_k \sum_{j,j'} a_j a_{j'}^* \delta_{jk} |A_{0,j}\rangle \langle A_{0,j'}| \delta_{j'k} \\ &= \sum_j |a_j|^2 |A_{0,j}\rangle \langle A_{0,j}|, \end{aligned} \quad (\text{S23})$$

similarly,

$$\rho_{B_0} = \text{Tr}_{B_1} [|\Psi_B\rangle \langle \Psi_B|] = \sum_k |b_k|^2 |B_{0,k}\rangle \langle B_{0,k}|. \quad (\text{S24})$$

Then the overlap  $S^2$  between the above two reduced density matrices are

$$\begin{aligned} S^2(\rho_{A_0}, \rho_{B_0}) &= \text{Tr}[\rho_{A_0} \rho_{B_0}] \\ &= \text{Tr} \left[ \sum_{j,k} |a_j|^2 |b_k|^2 |B_{0,k}\rangle \langle B_{0,k}| |A_{0,j}\rangle \langle A_{0,j}| \right] \\ &= \sum_l \sum_{j,k} |a_j|^2 |b_k|^2 \langle A_{0,l} | B_{0,k}\rangle \langle B_{0,k} | A_{0,j}\rangle \langle A_{0,j} | A_{0,l}\rangle \\ &= \sum_{j,k} |a_j|^2 |b_k|^2 |\langle A_{0,j} | B_{0,k}\rangle|^2, \end{aligned} \quad (\text{S25})$$

which agrees with the second term in the measurement probability in Eq. (S22). Therefore, we can reconstruct the overlap in (S25) using the measurement probability as

$$S^2(\rho_{A_0}, \rho_{B_0}) = 2 \text{Prob}[M = 0] - 1. \quad (\text{S26})$$

In the special case of  $\rho_{A_0} = \rho_{B_0}$ , the overlap as defined above reduces to evaluating the purity of a density matrix

$$\begin{aligned}
S^2(\rho_{A_0}, \rho_{A_0}) &= \text{Tr}[\rho_{A_0}^2] \\
&= \sum_{jk} |a_j|^2 |a_k|^2 |\langle A_{0,j} | A_{0,k} \rangle|^2 \\
&= \sum_{jk} |a_j|^2 |a_k|^2 \delta_{jk} \\
&= \sum_j |a_j|^4
\end{aligned} \tag{S27}$$

Since  $\sum_j |a_j|^2 = 1$ , and therefore  $S^2(\rho_{A_0}, \rho_{A_0}) \leq 1$ . When  $\rho_{A_0}$  corresponds to a pure state, there will be only one non-zero coefficient  $a_0 = 1$  and the rest being zero, leading to  $S^2(\rho_{A_0}, \rho_{A_0}) = 1$ . This agrees with the definition of purity.

### C. Connection to Quadratic Penalty

In our quantum bootstrap embedding algorithm, the quadratic constraint can be rewritten using the definition of overlap in the previous section as

$$\begin{aligned}
\text{Tr}[(\rho_{A_0} - \rho_{B_0})^2] &= \text{Tr}[(\rho_{A_0})^2] + \text{Tr}[(\rho_{B_0})^2] - 2 \text{Tr}[\rho_{A_0} \rho_{B_0}] \\
&= S^2(\rho_{A_0}, \rho_{A_0}) + S^2(\rho_{B_0}, \rho_{B_0}) - 2S^2(\rho_{A_0}, \rho_{B_0}).
\end{aligned} \tag{S28}$$

It is seen that the RHS of the above equation contains three **SWAP** tests: one for the overlap between  $\rho_{A_0}$  and  $\rho_{B_0}$  in (S25), and the other two for the purity of  $\rho_{A_0}$  and  $\rho_{B_0}$  respectively as in (S27).

## S5. EIGENVALUE EQUATIONS FOR THE QUADRATIC PENALTY METHOD

In Sec. 3.4 of the main text, we have seen that the quadratic constraint at the solution point has zero gradient with respect to the wave function parameters, and therefore does not satisfy the constraint qualification condition to use the Lagrange multiplier method for the optimization. Instead, we use a quadratic penalty method to perform the optimization of the loss function where an inherent eigenvalue equation with an effective bootstrap embedding potential  $V_{\text{BE}}$  is solved using a quantum eigensolver. The goal is to adjust  $V_{\text{BE}}$  such that two overlapping fragments match. In this section, we derive a rigorous expression for updating  $V_{\text{BE}}$  by taking the parameters in  $V_{\text{BE}}$  instead of the wave function as fundamental variable. For clarity, we keep the notation  $\lambda_B^{(A)}$  to refer to the penalty for fragment  $A$  and  $B$ , but all the penalty parameters are kept the same,  $\lambda_B^{(A)} = \lambda$ , as is also mentioned in the main text.

This can be achieved by taking the functional variation  $\delta V_{\text{BE}}$  and find the stationary point of  $\mathcal{L}_A$ . At the stationary point, we have

$$\delta \mathcal{L}_A = \sum_{ai\mu} \frac{\partial \mathcal{L}_A}{\partial C_{ai\mu}} \frac{\partial C_{ai\mu}}{\partial V_{\text{BE}}} \delta V_{\text{BE}} + \sum_{ai\mu} \frac{\partial \mathcal{L}_A}{\partial C_{ai\mu}^*} \frac{\partial C_{ai\mu}^*}{\partial V_{\text{BE}}} \delta V_{\text{BE}} = 0 \tag{S29}$$

for any  $\delta V_{\text{BE}}$ . This implies the equation of motion

$$\sum_{ai\mu} \frac{\partial \mathcal{L}_A}{\partial C_{ai\mu}} \frac{\partial C_{ai\mu}}{\partial V_{\text{BE}}} + \sum_{ai\mu} \frac{\partial \mathcal{L}_A}{\partial C_{ai\mu}^*} \frac{\partial C_{ai\mu}^*}{\partial V_{\text{BE}}} = 0. \tag{S30}$$

In the following, we derive separately  $\frac{\partial \mathcal{L}_A}{\partial C_{ai\mu}}$  (Sec. S5 A) and  $\frac{\partial C_{ai\mu}}{\partial V_{\text{BE}}}$  (Sec. S5 B), and then combine everything together in Sec. S5 C to obtain the overall gradient on how to updating the BE potential in the eigenvalue equation.

**A. Derivative  $\frac{\partial \mathcal{L}_A}{\partial C_{ai\mu}}$** 

Consider the derivative of  $\partial \mathcal{L}_A$  with respect to  $C_{ai\mu}$ :

$$\frac{d\mathcal{L}_A}{dC_{ai\mu}} = \frac{d}{dC_{ai\mu}} \left[ \langle H^{(A)} \rangle_A - \mathcal{E}(\langle I \rangle_A - 1) + \sum_{B \neq A}^{N_{frag}} \lambda_B^{(A)} \text{Tr}[(\rho_{\mathbb{E}_A} - \rho_{\mathbb{C}_B})^2] \right]. \quad (\text{S31})$$

Let's evaluate this term by term. The linear terms are easy:

$$\frac{d\langle H^{(A)} \rangle}{C_{bj\nu}^*} = \sum_{ai\mu} C_{ai\mu} \langle bj\nu | H^{(A)} | ai\mu \rangle, \quad (\text{S32})$$

$$\frac{d\mathcal{E}(\langle I \rangle - 1)}{C_{bj\nu}^*} = \mathcal{E} \sum_{ai\mu} C_{ai\mu} (I \otimes I \otimes I)_{ai\mu, bj\nu}, \quad (\text{S33})$$

$$\frac{d\text{Tr}[\rho_{\mathbb{E}_A} \rho_{\mathbb{C}_B}]}{dC_{bj\nu}^*} = \sum_i C_{bi\nu} \left( \sum_{a\mu} D_{ja\mu} D_{ia\mu}^* \right) = \sum_i (\rho_{\mathbb{C}_B})_{ji} C_{bi\nu}. \quad (\text{S34})$$

While the derivative involving quadratic term  $\frac{d\text{Tr}[\rho_{\mathbb{E}_A}^2]}{C_{ck\delta}^*}$  is a little tricky. First, note that

$$(\rho_{\mathbb{E}_A})^2 = \sum_{ii', jj'} \left( \sum_{a\mu} C_{ai\mu} C_{ai'\mu}^* \right) \left( \sum_{b\nu} C_{bj\nu} C_{bj'\nu}^* \delta_{i'j} |i\rangle \langle j'| \right), \quad (\text{S35})$$

from which we obtain

$$\text{Tr}[(\rho_{\mathbb{E}_A})^2] = \sum_{ij} \left( \sum_{a\mu} C_{ai\mu} C_{aj\mu}^* \right) \left( \sum_{b\nu} C_{bj\nu} C_{bi\nu}^* \right) \quad (\text{S36})$$

$$= \sum_{ij, ab, \mu\nu} (C_{ai\mu} C_{bj\nu}) (C_{aj\mu}^* C_{bi\nu}^*) \quad (\text{S37})$$

$$= \sum_{ij, ab, \mu\nu, i \neq j || a \neq b || \mu \neq \nu} (C_{ai\mu} C_{bj\nu}) (C_{aj\mu}^* C_{bi\nu}^*) + \sum_{ia\mu} (C_{ai\mu} C_{ai\mu}) (C_{ai\mu}^* C_{ai\mu}^*). \quad (\text{S38})$$

Note in order to take the derivative of the above with respect to  $C_{ck\delta}^*$ , we have separated the summation as two different terms because depending on whether the condition of  $a \neq b || j \neq i || \mu \neq \nu$  is met or not, the derivative will be different. Now evaluate the derivative of the above two terms separately, we have

$$\begin{aligned} \frac{d\text{Tr}[\rho_{\mathbb{E}_A}^2]}{dC_{ck\delta}^*} &= \sum_{ij, ab, \mu\nu, i \neq j || a \neq b || \mu \neq \nu} (C_{ai\mu} C_{bj\nu}) (C_{aj\mu}^* \delta_{bc} \delta_{ik} \delta_{\nu\delta} + C_{bi\nu}^* \delta_{ac} \delta_{jk} \delta_{\mu\delta}) \\ &\quad + \sum_{ia\mu} (C_{ai\mu} C_{ai\mu}) (2C_{ai\mu}^* \delta_{ac} \delta_{jk} \delta_{\mu\delta}) \end{aligned} \quad (\text{S39})$$

$$= \sum_{ja\mu, k \neq j || a \neq c || \mu \neq \delta} (C_{ak\mu} C_{cj\delta}) C_{aj\mu}^* + \sum_{ib\nu, i \neq k || b \neq c || \nu \neq \delta} (C_{ci\delta} C_{bk\nu}) C_{bi\nu}^* + 2C_{ck\delta}^2 C_{ck\delta}^*. \quad (\text{S40})$$

Now in each of the above terms, combine a  $C$  and a  $C^*$  we can recover some elements of  $\rho_{\mathbb{E}_A}$ . For example, in the first term we have

$$\sum_{ja\mu, k \neq j || a \neq c || \mu \neq \delta} (C_{ak\mu} C_{cj\delta}) C_{aj\mu}^* = \sum_{j, k \neq j || a \neq c || \mu \neq \delta} \left( \sum_{a\mu} C_{ak\mu} C_{aj\mu}^* \right) C_{cj\delta} \quad (\text{S41})$$

$$= \sum_{j, k \neq j || a \neq c || \mu \neq \delta} \left( \rho_{\mathbb{E}_A}^{(a\mu)} \right)_{kj} C_{cj\delta}, \quad (\text{S42})$$

where in the last line the superscript  $(a\mu)$  on  $\rho_{\mathbb{E}_A}^{(a\mu)}$  simply means the implicit summation is over dummy variables  $a\mu$ .

With this notation, we can collect all terms in  $\frac{d \text{Tr}[\rho_{\mathbb{E}_A}^2]}{C_{ck\delta}^*}$  and write it as

$$\frac{d \text{Tr}[\rho_{\mathbb{E}_A}^2]}{dC_{bj\nu}^*} = 2 \sum_{i,k \neq i || b \neq c || \nu \neq \delta} \left( \rho_{\mathbb{E}_A}^{(b\nu)} \right)_{ki} C_{ci\delta} + 2 (\rho_A)_{ck\delta, ck\delta} C_{ck\delta}, \quad (\text{S43})$$

which consists of two terms. With the derivative of  $\text{Tr}[\rho_{\mathbb{E}_A}^2]$ , we can combine this with the derivative of  $\text{Tr}[\rho_{\mathbb{E}_A} \rho_{\mathbb{C}_B}]$  to get

$$\begin{aligned} \frac{d \text{Tr}[(\rho_{\mathbb{E}_A} - \rho_{\mathbb{C}_B})^2]}{dC_{ck\delta}^*} &= \frac{d \text{Tr}[(\rho_{\mathbb{E}_A})^2]}{C_{ck\delta}^*} - 2 \frac{d \text{Tr}[\rho_{\mathbb{E}_A} \rho_{\mathbb{C}_B}]}{C_{ck\delta}^*} \\ &= 2 \sum_{i,k \neq i || b \neq c || \nu \neq \delta} \left( \rho_{\mathbb{E}_A}^{(b\nu)} - \rho_{\mathbb{C}_B}^{(b\nu)} \right)_{ki} C_{ci\delta} + 2 [(\rho_A)_{ck\delta, ck\delta} - (\rho_B)_{kc\delta, kc\delta}] C_{ck\delta}. \end{aligned} \quad (\text{S44})$$

Notice the subscripts of  $\rho_B$  on the last term of RHS is in different order as compared to  $\rho_A$  due to the distinction between center and edge sites.

Combine this with the derivative of the other terms, we obtain the following eigenvalue equation

$$\begin{aligned} \frac{d\mathcal{L}_A}{dC_{ck\delta}^*} &= \sum_{ai\mu} C_{ai\mu} \langle ck\delta | H^{(A)} | ai\mu \rangle + \mathcal{E} \sum_{ai\mu} C_{ai\mu} (I \otimes I \otimes I)_{ck\delta, ai\mu} \\ &+ 2\lambda_B^{(A)} \left[ \sum_{i, (a, i, \mu) \neq (c, k, \delta)} \left( \rho_{\mathbb{E}_A}^{(a\mu)} - \rho_{\mathbb{C}_B}^{(a\mu)} \right)_{ki} C_{ci\delta} + [(\rho_A)_{ck\delta, ck\delta} - (\rho_B)_{kc\delta, kc\delta}] C_{ck\delta} \right] = 0, \quad \forall c, k, \delta. \end{aligned} \quad (\text{S45})$$

This equation seems to be difficult to rewrite into matrix notation, but actually they are easy if written under the full density matrix of fragment A and B. In terms of full density matrices of the fragments, the first term in the effective potential is

$$\sum_{i, (a, i, \mu) \neq (c, k, \delta)} \left( \rho_{\mathbb{E}_A}^{(a\mu)} - \rho_{\mathbb{C}_B}^{(a\mu)} \right)_{ki} C_{ci\delta} = \sum_{ai\mu, (a, i, \mu) \neq (c, k, \delta)} [(\rho_A)_{ak\mu, ai\mu} - (\rho_B)_{ka\mu, ia\mu}] C_{ci\delta}. \quad (\text{S46})$$

It can also be recognized that the second term in the effective potential is essentially

$$[(\rho_A)_{ck\delta, ck\delta} - (\rho_B)_{kc\delta, kc\delta}] C_{ck\delta} = \sum_{ai\mu, (a, i, \mu) = (c, k, \delta)} [(\rho_A)_{ak\mu, ai\mu} - (\rho_B)_{ka\mu, ia\mu}] C_{ci\delta}. \quad (\text{S47})$$

Substitute the above two equations into Eq. (S45), we have

$$\begin{aligned} \frac{d\mathcal{L}_A}{dC_{ck\delta}^*} &= \sum_{ai\mu} C_{ai\mu} \langle ck\delta | H^{(A)} | ai\mu \rangle + \mathcal{E} \sum_{ai\mu} C_{ai\mu} (I \otimes I \otimes I)_{ck\delta, ai\mu} \\ &+ 2\lambda_B^{(A)} \left[ \left( \sum_{ai\mu, (a, i, \mu) \neq (c, k, \delta)} + \sum_{ai\mu, (a, i, \mu) = (c, k, \delta)} \right) [(\rho_A)_{ak\mu, ai\mu} - (\rho_B)_{ka\mu, ia\mu}] C_{ci\delta} \right] = 0, \quad \forall c, k, \delta \\ &= \sum_{ai\mu} C_{ai\mu} \langle ck\delta | H^{(A)} | ai\mu \rangle + \mathcal{E} \sum_{ai\mu} C_{ai\mu} (I \otimes I \otimes I)_{ck\delta, ai\mu} + 2\lambda_B^{(A)} \sum_{ai\mu} C_{ci\delta} [(\rho_A)_{ak\mu, ai\mu} - (\rho_B)_{ka\mu, ia\mu}] \end{aligned} \quad (\text{S48})$$

$$= \sum_{ai\mu} \langle ck\delta | H^{(A)} | ai\mu \rangle C_{ai\mu} + \mathcal{E} \sum_{ai\mu} (I \otimes I \otimes I)_{ck\delta, ai\mu} C_{ai\mu} + 2\lambda_B^{(A)} \sum_i (\rho_{\mathbb{E}_A} - \rho_{\mathbb{C}_B})_{ki} C_{ci\delta} = 0, \quad \forall c, k, \delta \quad (\text{S49})$$

## B. Derivative $\frac{\partial C_{ai\mu}}{\delta V_{BE}}$

In this section, we focus on deriving  $\frac{\partial C_{ai\mu}}{\delta V_{BE}}$  or  $\frac{\partial C_{ai\mu}^*}{\delta V_{BE}}$ .

Use wave function perturbation theory on the following eigenvalue equation

$$(H^{(A)} + V_{BE}) |\psi_{A,n}\rangle = -\mathcal{E}_n^{(A)} |\psi_{A,n}\rangle, \quad (S50)$$

where  $n$  labels different eigenstates. Now given a small variation of  $V_{BE}$ , the eigenstates and eigenenergies will change. To 1st-order perturbation, we can write the change of each eigenstate as

$$\delta |\psi_{A,n}\rangle = \sum_{n' \neq n} \frac{\langle \psi_{A,n'} | (\delta V_{BE}) | \psi_{A,n} \rangle}{\mathcal{E}_n^{(A)} - \mathcal{E}_{n'}^{(A)}} |\psi_{A,n'}\rangle. \quad (S51)$$

This is a change on the eigenstate, and not yet exact what we want (we want change on the coefficients in front of basis vector,  $C_{ai\mu}^{(n)}$ , note the superscript labels the  $n$ -th eigenstate). To do this, let's further write the eigenstates in terms of all the coefficients,

$$|\psi_{A,n}\rangle = \sum_{ai\mu} C_{ai\mu}^{(n)} |ai\mu\rangle, \quad (S52)$$

then the above equation becomes an array of coupled-system of equations:

$$\sum_{ai\mu} dC_{ai\mu}^{(n)} |ai\mu\rangle = \sum_{n' \neq n} \sum_{a''i''\mu'', a'i'\mu', ai\mu} C_{a'i'\mu'}^{(n')*} C_{ai\mu}^{(n)} \frac{\langle a'i'\mu' | (\delta V_{BE}) | ai\mu \rangle}{\mathcal{E}_n^{(A)} - \mathcal{E}_{n'}^{(A)}} C_{a''i''\mu''}^{(n')} |a''i''\mu''\rangle. \quad (S53)$$

Multiply both sides with  $\langle a'''i'''\mu'''|$ , we arrives at the following equation on the coefficients after relabeling the  $ai\mu$  index

$$dC_{ai\mu}^{(n)} = \sum_{n' \neq n} \sum_{a''i''\mu'', a'i'\mu'} C_{a''i''\mu''}^{(n')*} C_{a'i'\mu'}^{(n)} \frac{\langle a''i''\mu'' | (\delta V_{BE}) | a'i'\mu' \rangle}{\mathcal{E}_n^{(A)} - \mathcal{E}_{n'}^{(A)}} C_{ai\mu}^{(n')}, \quad (S54)$$

for any index  $(a, i, \mu)$ .

To further simplify the above equation, we introduce parametrization of  $\delta V_{BE}$  as linear combination of local potentials on the edge sites  $V_{BE} = \sum_{\alpha=0}^{4^m} v_{\alpha} I \otimes \Sigma_{\alpha} \otimes I$ , where the first and the last identity operators act on the center and the bath sites by definition. Therefore, a functional variation of  $V_{BE}$  can be parametrized as a small change in the scalar coefficients  $v_{\alpha}$

$$\delta V_{BE} = \sum_{\alpha=0}^{4^m} dv_{\alpha} I \otimes \Sigma_{\alpha} \otimes I, \quad (S55)$$

and the matrix elements are

$$\langle a''i''\mu'' | (\delta V_{BE}) | a'i'\mu' \rangle = \delta_{a'a''} \delta_{\mu'\mu''} \sum_{\alpha=0}^{4^m} \langle i'' | \Sigma_{\alpha} | i' \rangle dv_{\alpha}. \quad (S56)$$

This leads to the simplified expression for  $dC_{ai\mu}^{(n)}/\delta V_{BE}$

$$\frac{dC_{ai\mu}^{(n)}}{\delta V_{BE}} = \sum_{\alpha=0}^{4^m} \frac{dC_{ai\mu}^{(n)}}{dv_{\alpha}} = \sum_{n' \neq n} \sum_{i'', a'i'\mu'} C_{a'i'\mu'}^{(n')*} C_{ai\mu}^{(n)} \frac{\sum_{\alpha=0}^{4^m} \langle i'' | \Sigma_{\alpha} | i' \rangle}{\mathcal{E}_n^{(A)} - \mathcal{E}_{n'}^{(A)}} C_{ai\mu}^{(n')}. \quad (S57)$$

In particular, for the ground eigenstate, we have (omitting the superscript  $(0)$ )

$$\frac{dC_{ck\delta}^*}{\delta V_{BE}} = \sum_{\alpha=0}^{4^m} \frac{dC_{ck\delta}^*}{dv_{\alpha}} = \sum_{n' \neq 0} \sum_{i', ai\mu} C_{ai\mu}^{(n')} C_{ai\mu}^* \frac{\sum_{\alpha=0}^{4^m} \langle i | \Sigma_{\alpha} | i' \rangle}{\mathcal{E}_0^{(A)} - \mathcal{E}_{n'}^{(A)}} C_{ck\delta}^{(n')*}. \quad (S58)$$

### C. Gradient of Cost Function versus BE Potential

Now we are ready to put everything together to obtain a final expression for the gradient of the cost function versus the BE potential.

Substitute Eq. (S58) and Eq. (S49) into (S30), we obtain

$$\begin{aligned} \sum_{ck\delta} \frac{d\mathcal{L}_A}{dC_{ck\delta}^*} \frac{dC_{ck\delta}^*}{\delta V_{BE}} &= \sum_{ck\delta} \left[ \sum_{ai\mu} \langle ck\delta | H^{(A)} | ai\mu \rangle C_{ai\mu} + \mathcal{E}_0^{(A)} \sum_{ai\mu} (I \otimes I \otimes I)_{ck\delta, ai\mu} C_{ai\mu} + 2\lambda_B^{(A)} \sum_i (\rho_{\mathbb{E}_A} - \rho_{\mathbb{C}_B})_{ki} C_{ci\delta} \right] \\ &\times \left[ \sum_{n' \neq 0} \sum_{i', ai\mu} C_{ai'\mu}^{(n')} C_{ai\mu}^* \frac{\sum_{\alpha=0}^{4^m} \langle i | \Sigma_\alpha | i' \rangle}{\mathcal{E}_0^{(A)} - \mathcal{E}_{n'}^{(A)}} C_{ck\delta}^{(n')*} \right] = 0. \end{aligned} \quad (\text{S59})$$

Writing this in matrix form,

$$\begin{aligned} &\sum_{ck\delta} \left\{ (\mathbf{H}^{(A)} \mathbf{C})_{ck\delta} + (\mathcal{E}_0^{(A)} \mathbf{C})_{ck\delta} + 2\lambda_B^{(A)} [(\mathbf{I} \otimes (\rho_{\mathbb{E}_A} - \rho_{\mathbb{C}_B}) \otimes \mathbf{I}) \mathbf{C}]_{ck\delta} \right\} \\ &\times \left[ \sum_{n' \neq 0} [\mathbf{C}^\dagger (\mathbf{I} \otimes \sum_{\alpha=0}^{4^m} \mathbf{W}_\alpha^{(n')} \otimes \mathbf{I}) \mathbf{C}^{(n')}] \mathbf{C}^{(n')*} \right]_{ck\delta} = 0. \end{aligned} \quad (\text{S60})$$

or

$$\sum_{n' \neq 0} \left[ \mathbf{C}^\dagger (\mathbf{I} \otimes \sum_{\alpha=0}^{4^m} \mathbf{W}_\alpha^{(n')} \otimes \mathbf{I}) \mathbf{C}^{(n')} \right] \times \left[ \mathbf{C}^{(n')\dagger} \left( \mathbf{H}^{(A)} + \mathcal{E}_0^{(A)} + 2\lambda_B^{(A)} (\mathbf{I} \otimes (\rho_{\mathbb{E}_A} - \rho_{\mathbb{C}_B}) \otimes \mathbf{I}) \right) \mathbf{C} \right] = 0. \quad (\text{S61})$$

where  $\mathbf{W}_\alpha^{(n')}_{ii'} = \frac{\langle i | \Sigma_\alpha | i' \rangle}{\mathcal{E}_0^{(A)} - \mathcal{E}_{n'}^{(A)}}$ . Writing this with respect to each parameter  $v_\alpha$  in  $V_{BE}$ , we have

$$\frac{d\mathcal{L}_A}{dv_\alpha} = \sum_{n' \neq 0} \left[ \mathbf{C}^\dagger (\mathbf{I} \otimes \mathbf{W}_\alpha^{(n')} \otimes \mathbf{I}) \mathbf{C}^{(n')} \right] \times \left[ \mathbf{C}^{(n')\dagger} \left( \mathbf{H}^{(A)} + \mathcal{E}_0^{(A)} + 2\lambda_B^{(A)} (\mathbf{I} \otimes (\rho_{\mathbb{E}_A} - \rho_{\mathbb{C}_B}) \otimes \mathbf{I}) \right) \mathbf{C} \right], \quad \forall \alpha \in [0, 4^m]. \quad (\text{S62})$$

From this gradient, we may update all the fundamental parameters  $\{\lambda_B^{(A)}, v_\alpha\}$  using gradient descent (or other update scheme) to minimize the Lagrangian, as is typically performed in optimization. However, to compute this gradient exactly in (S62), it is required that all the eigenstates are known (not only the ground state) which is clearly very costly and not that useful. Nevertheless, it serves as a good starting point to develop *approximated* updating scheme. One possible approximation is to truncate the summation over  $n'$  to only a low energy subspace. More efficient approximations are left for future investigation.

### S6. SAMPLE COMPLEXITY FOR ESTIMATING THE OVERLAP FROM TOMOGRAPHY

We have seen that the linear and quadratic constraints are equivalent in Sec. S3, and presented that an efficient quantum circuit based on SWAP test in Sec. S4. In this section, we derive the sample complexity of estimating the RDM mismatch by naively sampling individual RDM element from tomography, to demonstrate the advantage of using the SWAP test in quadratic matching.

Recall that the quadratic mismatch between two RDMs reduces to the sum of element-wise distance (squared) of their individual RDM elements from (S18)

$$S^2(\rho_A, \rho_B) = \sum_{\alpha=1}^{4^m-1} (\langle \Sigma_\alpha \rangle_A - \langle \Sigma_\alpha \rangle_B)^2. \quad (\text{S63})$$

where  $m$  is the number of qubits in the overlapping region.

Let's denote the true value of

$$\lim_{\text{sample size} \rightarrow \infty} \langle \Sigma_\alpha \rangle_X = R_\alpha^{(X)} \quad (\text{S64})$$

for  $X = A, B$ . Then, in tomography the estimate uncertainty of  $\{R_\alpha^{(A)}, R_\alpha^{(B)}\}$  will propagate to the uncertainty of  $S^2$  via

$$\text{var}(S^2) = \mathbf{J} \cdot \begin{bmatrix} C_{\{R_\alpha^{(A)}\}} & \\ & C_{\{R_\alpha^{(B)}\}} \end{bmatrix} \cdot \mathbf{J}^T, \quad (\text{S65})$$

where  $\mathbf{J} = \nabla_{\{R_\alpha^{(A)}, R_\alpha^{(B)}\}} S^2 = [\frac{\partial S^2}{\partial R_1^{(A)}}, \frac{\partial S^2}{\partial R_2^{(A)}}, \dots, \frac{\partial S^2}{\partial R_{4^m-1}^{(A)}}, \frac{\partial S^2}{\partial R_1^{(B)}}, \frac{\partial S^2}{\partial R_2^{(B)}}, \dots, \frac{\partial S^2}{\partial R_{4^m-1}^{(B)}}]$  is the Jacobian,  $C_{\{R^{(A)}\}}$  and  $C_{\{R^{(B)}\}}$  are the co-variance matrix of the RDM elements.  $\text{var}(\cdot)$  denotes the variance.

Note that  $C_{\{R^{(A)}\}}$  and  $C_{\{R^{(B)}\}}$  will be system-dependent, and for now let us assume there is not co-variance between individual elements of  $\rho_A$  and  $\rho_B$ , and therefore  $C_{\{R^{(A)}\}}$  and  $C_{\{R^{(B)}\}}$  will be diagonal with diagonal elements being the variance of each RDM element.

Moreover, by substituting (S63) into  $\mathbf{J}$ , we can explicitly evaluate

$$\begin{aligned} \mathbf{J}_{A,\alpha} &= \frac{\partial S^2}{\partial R_\alpha^{(A)}} = 2 \left( R_\alpha^{(A)} - R_\alpha^{(B)} \right), \\ \mathbf{J}_{B,\alpha} &= \frac{\partial S^2}{\partial R_\alpha^{(B)}} = -2 \left( R_\alpha^{(A)} - R_\alpha^{(B)} \right). \end{aligned} \quad (\text{S66})$$

This gives

$$\text{var}(S^2) = 4 \sum_{i=1}^{4^m-1} \left( R_\alpha^{(A)} - R_\alpha^{(B)} \right)^2 \left[ \text{var}(R_\alpha^{(A)}) + \text{var}(R_\alpha^{(B)}) \right]. \quad (\text{S67})$$

Now assume that each element of the RDM is estimated by the same amount of samples  $N_{\text{samp},0}$ , then from binomial distribution, the variance of each  $R_\alpha^{(A)}$  and  $R_\alpha^{(B)}$  is

$$\text{var}(R_\alpha^{(X)}) = \frac{R_\alpha^{(X)}(1 - R_\alpha^{(X)})}{N_{\text{samp},0}}, \quad \forall X = A, B. \quad (\text{S68})$$

Substitute this into (S67), we have

$$\text{var}(S^2) = \frac{4DS^2}{N_{\text{samp},0}}, \quad (\text{S69})$$

where  $D$  is a system-dependent constant

$$D = \frac{\sum_{\alpha=1}^{4^m-1} \left( R_\alpha^{(A)} - R_\alpha^{(B)} \right)^2 \left( R_\alpha^{(A)}(1 - R_\alpha^{(A)}) + R_\alpha^{(B)}(1 - R_\alpha^{(B)}) \right)}{\sum_{\alpha=1}^{4^m-1} \left( R_\alpha^{(A)} - R_\alpha^{(B)} \right)^2} \quad (\text{S70})$$

Given a target accuracy  $\epsilon$  on  $S$ , then  $\text{var}(S^2) = (2S\epsilon)^2$ , from the above equation we can solve to obtain the required number of samples as for each individual RDM elements

$$N_{\text{samp},0} = \frac{D}{\epsilon^2}. \quad (\text{S71})$$

There are  $4^n - 1$  elements for  $n$ -qubit overlapping region, leading to an overall sampling complexity of

$$N_{\text{samp}}^{\text{TMG}} = \mathcal{O}(e^n) \cdot N_{\text{samp},0} = \mathcal{O}(e^n) \frac{D}{\epsilon^2}, \quad (\text{S72})$$

for estimating the overlap to  $\epsilon$  accuracy from density matrix tomography. The reason why  $\mathcal{O}(e^n)$  instead of naive

$4^n - 1$  is because there are commuting Pauli operators that can be estimated simultaneously. However, the exponential scaling in terms of the number of overlapping qubits  $n$  remains.

As is mentioned in the main text, overlaps between density matrices are not low-rank observables, so the sampling complexity of estimating it is likely to be high. However, more efficient sampling schemes may exist. For example, by sampling the differences in the RDMs between the current and the previous BE iterations, the sampling complexity could be much better than exponential. One simple way of doing this is to use the diagonal basis of the previous iteration as the measurement basis in the current iteration to perform the RDM sampling. We leave this for future investigation.

## S7. DETAILS OF QUANTUM AMPLITUDE ESTIMATION AND QUADRATIC SPEEDUP

In this section, we describe in detail how a quantum amplitude estimation can be implemented by combining an oblivious amplitude amplification (Sec. S7A) with a binary search algorithm (Sec. S7B). We then outline how a binary search derive the sample complexity needed to achieve a constant precision  $\epsilon$  in the overlap in our coherent matching algorithm and compare that with a classical incoherent sampling estimation scheme, demonstrating a quadratic speedup of the former (Sec. S7C).

### A. Amplitude Amplification

From Theorem 2 of Ref. [4], it is shown that given a state preparation process  $U$  from an initial state  $|B_0\rangle$ , the overlap  $a$  of this prepared state with another state  $|A_0\rangle$ , i.e.,  $a := \langle A_0 | U | B_0 \rangle$ , can be transformed by a  $d$ -degree polynomial  $P(a)$  such that  $|1 - P(a)| < \delta$  using rotations  $A_\phi = e^{i\phi|A_0\rangle\langle A_0|}$  and  $B_\phi = e^{i\phi|B_0\rangle\langle B_0|}$  by the following quantum circuit

$$P(a) = \langle A_0 | \left[ \prod_{j=1}^{d/2} U B_{\phi_{2j-1}} U^\dagger A_{\phi_{2j}} \right] U | B_0 \rangle, \quad (\text{S73})$$

where  $d = \mathcal{O}(\frac{1}{a} \log(1/\delta))$ , and the rotation angles  $\phi_{2j}$  and  $\phi_{2j-1}$  can be efficiently computed classically. This is a generalization of Grover's search algorithm where the rotation  $B_\phi$  is similar to the diffusion operator (reflection about the average), and  $A_\phi$  is analogous to the Grover's reflection about the target state. The difference is that the rotation angles  $\phi$ 's can be fractions of  $\pi$  and is thus more general which combines the optimality of Grover's algorithm for unstructured search and the fixed-point property [5].

In our case, denote  $S = |\langle \Psi^{\mathbb{E}} | \Phi^{\mathbb{C}} \rangle|$  as the overlap of the edge of the first fragment and center of the second fragment in their ground states, and choose the following for state  $|A_0\rangle$  and  $|B_0\rangle$

$$|A_0\rangle = \frac{1}{\sqrt{2(1+S^2)}} |0\rangle \left( |\Psi^{\mathbb{E}}\rangle |\Psi^{\mathbb{E}}\rangle |\Phi^{\mathbb{C}}\rangle |\Phi^{\mathbb{C}}\rangle + |\Psi^{\mathbb{E}}\rangle |\Phi^{\mathbb{C}}\rangle |\Psi^{\mathbb{E}}\rangle |\Phi^{\mathbb{C}}\rangle \right) \quad (\text{S74})$$

$$|B_0\rangle = |0\rangle |\Psi_T^{\mathbb{E}}\rangle |\Psi_T^{\mathbb{E}}\rangle |\Phi_T^{\mathbb{C}}\rangle |\Phi_T^{\mathbb{C}}\rangle, \quad (\text{S75})$$

where  $|B_0\rangle$  is the input trial states (thus the subscript ‘‘T’’) for the quantum eigensolver, while  $|A_0\rangle$  is the symmetric subspace of the SWAP test. Let  $U$  be the state preparation circuit (in our case the two quantum eigensolver + the SWAP test) given by Fig. S2.

Given these choices, it can be verified that the

$$U | B_0 \rangle = a | A_0 \rangle + \sqrt{1 - a^2} | A_\perp \rangle \quad (\text{S76})$$

where

$$a = \langle A_0 | U | B_0 \rangle = \sqrt{\frac{1 + S^2}{2}}, \quad (\text{S77})$$

and

$$|A_\perp\rangle = \frac{1}{\sqrt{2(1-S^2)}} |1\rangle \left( |\Psi^{\mathbb{E}}\rangle |\Psi^{\mathbb{E}}\rangle |\Phi^{\mathbb{C}}\rangle |\Phi^{\mathbb{C}}\rangle - |\Psi^{\mathbb{E}}\rangle |\Phi^{\mathbb{C}}\rangle |\Psi^{\mathbb{E}}\rangle |\Phi^{\mathbb{C}}\rangle \right). \quad (\text{S78})$$

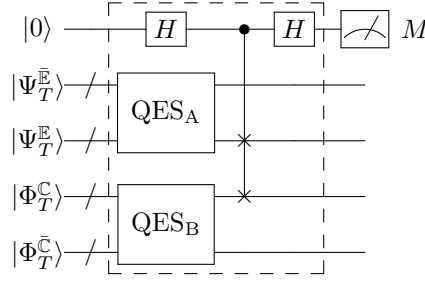

FIG. S2: Quantum circuit to estimate the ground state overlap between subsystems of two fragments, composed of two quantum eigensolver (QES) for two fragments ground state wave function followed by a **SWAP** test. The circuit in the dashed box is  $U$  in Eq. (S73) which will be repeated multiple times during the amplitude amplification process as will be discussed in the following.

Note the choice of  $|A_\perp\rangle$  has a lot of degrees of freedom, as long as it is normalized and orthogonal to  $|A_0\rangle$ . In particular,  $|A_\perp\rangle = |1\rangle|\Psi\rangle$  for any  $|\Psi\rangle$  (with support on the two system registers) will work as long as the ancilla qubit is at state  $|1\rangle$ .

Moreover, we choose  $|B_\perp\rangle$  such that

$$U|B_\perp\rangle = -a|A_\perp\rangle + \sqrt{1-a^2}|A_0\rangle \quad (\text{S79})$$

which leads to an explicit expression for  $|B_\perp\rangle$

$$\begin{aligned} |B_\perp\rangle &= -aU^{-1}|A_\perp\rangle + \sqrt{1-a^2}U^{-1}|A_0\rangle \\ &= \frac{1}{2}|0\rangle \otimes \\ &\quad \left[ -\sqrt{\frac{1+S^2}{1-S^2}} \left( |\Psi_T^{\bar{E}}\rangle |\Psi_T^E\rangle |\Phi_T^C\rangle |\Phi_T^{\bar{C}}\rangle - |\Psi_T^{\bar{E}}\rangle |\Phi_T^C\rangle |\Psi_T^E\rangle |\Phi_T^{\bar{C}}\rangle \right) \right. \\ &\quad \left. + \sqrt{\frac{1-S^2}{1+S^2}} \left( |\Psi_T^{\bar{E}}\rangle |\Psi_T^E\rangle |\Phi_T^C\rangle |\Phi_T^{\bar{C}}\rangle + |\Psi_T^{\bar{E}}\rangle |\Phi_T^C\rangle |\Psi_T^E\rangle |\Phi_T^{\bar{C}}\rangle \right) \right]. \end{aligned} \quad (\text{S80})$$

It then follows that  $\{|A_0\rangle, |A_\perp\rangle\}$  and  $\{|B_0\rangle, |B_\perp\rangle\}$ , each forms a 2-dimensional subspace where  $U$  can be expanded upon

$$\begin{aligned} U &= a|A_0\rangle\langle B_0| + \sqrt{1-a^2}|A_\perp\rangle\langle B_0| \\ &\quad - a|A_\perp\rangle\langle B_\perp| + \sqrt{1-a^2}|A_0\rangle\langle B_\perp| \end{aligned} \quad (\text{S81})$$

$$= \begin{bmatrix} a & \sqrt{1-a^2} \\ \sqrt{1-a^2} & -a \end{bmatrix}. \quad (\text{S82})$$

Given access to  $A_\phi$  and  $B_\phi$ , the rest of amplitude amplification follows the same as Ref. [4] by using Eq. (S73).

We should note that the rotation  $B_\phi$  is easy to construct from

$$B_\phi = e^{i\phi|B_0\rangle\langle B_0|} = U_T e^{i\phi|0\rangle\langle 0|^{\otimes}} U_T^\dagger, \quad (\text{S83})$$

because  $U_T$  is a known unitary that can prepare the initial trial state (for example Hartree-Fock state) from the zero state

$$|0\rangle \otimes |\Psi_T^{\bar{E}}\rangle |\Psi_T^E\rangle |\Phi_T^C\rangle |\Phi_T^{\bar{C}}\rangle = U_T |0\rangle^{\otimes}. \quad (\text{S84})$$

At first glance, the rotation  $A_\phi$  seems to be more difficult and it requires an oracle to prepare  $|A_0\rangle$  from the zero state

$$|A_0\rangle = V|0\rangle^{\otimes}, \quad (\text{S85})$$

such that  $A_\phi = e^{i\phi|A_0\rangle\langle A_0|} = V e^{i\phi|0\rangle\langle 0|} V^\dagger$ . However, because the SWAP test entangles the symmetric and anti-symmetric subspace of the two system register separately with  $|0\rangle$  and  $|1\rangle$  state of the ancilla, we can simply choose

$$A_\phi = e^{i\phi(|0\rangle\langle 0| - |1\rangle\langle 1|) \otimes I^\otimes} = e^{i\phi Z \otimes I^\otimes}, \quad (\text{S86})$$

which is just a single-qubit  $Z$  rotation on the ancilla, and the identity operator  $I^\otimes$  has support on the two system registers. It can be readily verified that when applying  $A_\phi$  to a linear combination of  $|A_0\rangle$  and  $|A_\perp\rangle$  that

$$\begin{aligned} A_\phi(c_0|A_0\rangle + c_1|A_\perp\rangle) &= e^{i\phi(|0\rangle\langle 0| - |1\rangle\langle 1|) \otimes I^\otimes} (c_0|0\rangle \otimes |\Psi_{A_0}\rangle + c_1|1\rangle \otimes |\Psi_{A_\perp}\rangle) \\ &= c_0 e^{i\phi} |0\rangle \otimes |\Psi_{A_0}\rangle + c_1 e^{-i\phi} |1\rangle \otimes |\Psi_{A_\perp}\rangle \\ &= e^{i\phi} c_0 |A_0\rangle + e^{-i\phi} c_1 |A_\perp\rangle, \end{aligned} \quad (\text{S87})$$

which imposes a relative phase of  $2\phi$  between the target state  $|A_0\rangle$  and the unwanted state  $|A_\perp\rangle$  as desired.

With these construction, the overall quantum circuit for the amplitude amplification is given in Fig. S3. with the

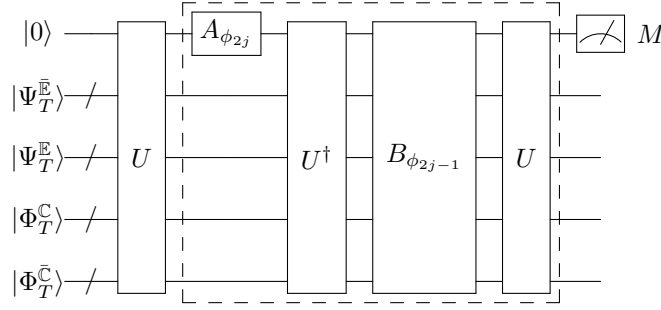

FIG. S3: Quantum circuit for fixed-point oblivious amplitude amplification of the coherent quantum matching. The quantum gates in dashed box corresponds to the gates in bracket of Eq. (S73) which needs to be repeated by  $d/2$  times, where  $d$  will be determined by the slope of the amplification polynomial  $\frac{1}{\Delta_k}$  (more about this in the next section).

state prep circuit  $U$  given in Fig. S2, and the rotation  $A_{\phi_{2j}}$  and  $B_{\phi_{2j-1}}$  defined in Eq. (S86) and (S83) respectively. Note that this circuit requires  $U^\dagger$  which means the two quantum eigensolvers in  $U$  has to be run in backwards, which is certainly possible for solvers such as QPE and VQE.

### B. Estimate the Amplitude from Binary Search

The above amplitude amplification can be combined with a binary search algorithm to estimate the magnitude of the amplitude  $a = \sqrt{\frac{1+S^2}{2}}$  up to precision  $\epsilon = \frac{1}{2^n}$  in a bit-by-bit fashion.

Denote a binary representation of the amplitude  $a$  as

$$a := [b_{n-1}b_{n-2}\dots b_1b_0] = \frac{1}{2^n} (b_{n-1}2^{n-1} + b_{n-2}2^{n-2} + \dots + b_0). \quad (\text{S88})$$

We perform the following two steps repeatedly to determine  $b_k$  for  $k = n-1, n-2, \dots, 1, 0$ :

1. Perform a fixed-point amplitude amplification using a polynomial in Ref. [4] with slope  $\frac{1}{\Delta_k}$  (this determines the depth of the circuit  $d$  as in Fig. S3) and precision  $\epsilon$ , where  $\Delta_k$  is determined from all previous estimations on  $b_{n-1}, \dots, b_{k+1}$  by

$$\Delta_k = \frac{\sqrt{2}}{2^n} \left( \sum_{l=k+1}^{n-1} b_l 2^l + 2^k \right). \quad (\text{S89})$$

2. Measure the ancilla of the SWAP test by collecting  $N_\epsilon = \lceil \frac{2}{\epsilon} \rceil$  samples and then set  $b_k$  to the expectation value of the estimated outcome,  $b_k = \langle M \rangle$ .

It can be verified that this protocol works because each time after the amplitude amplification, if  $\langle M \rangle = 1$ , then the amplitude ends up in the interval  $[0.b_{n-1}b_{n-2}\cdots b_{k+1}1, 0.b_{n-1}b_{n-2}\cdots b_{k+1}1 + \frac{1}{2^{n-k}}]$ ; otherwise if  $\langle M \rangle = 0$ , then the amplitude ends up in the interval  $[0.b_{n-1}b_{n-2}\cdots b_{k+1}0, 0.b_{n-1}b_{n-2}\cdots b_{k+1}1]$ . We choose  $N_\epsilon$  to be large enough such that it is sufficient to tell if the amplified amplitude is within the range of  $[1 - \epsilon, 1]$  with high probability. For a Bernoulli distribution with  $p \in [(1 - \epsilon)^2, 1]$ , we require the standard deviation of the estimation for amplitude to be roughly  $\epsilon$ , i.e.

$$\Delta a = \left| \frac{da}{dp} \right| \Delta p = \frac{1}{2} \sqrt{\frac{(1-p)}{N_\epsilon}} = \epsilon, \quad (\text{S90})$$

which gives

$$N_\epsilon = \frac{(1-p)}{4\epsilon^2} = \frac{1 - (1-\epsilon)^2}{4\epsilon^2} = \frac{1}{2\epsilon} - \frac{1}{4}. \quad (\text{S91})$$

Therefore, a choice of  $N_\epsilon = \lceil \frac{1}{2\epsilon} \rceil$  suffices.

### C. Quadratic Speedup

We demonstrate the quantum speedup due to amplitude amplification (AA) by estimate the sample complexity required to achieve a constant precision on estimating  $a$ .

We first estimate the total number of samples in the SWAP test + amplitude estimation (AE) approach by combining AA and binary search. For each digit  $b_k$ , each sample takes a total of  $\frac{1}{\Delta_k} \log(\frac{1}{\epsilon})$  queries to the eigensolver in the amplitude amplification for  $\Delta_k$  in Eq. (S89), and we need  $N_\epsilon$  (Eq. (S91)) samples to estimate whether the amplified amplitude is within the range of  $[1 - \epsilon, 1]$ , which gets us to the number of queries to the eigensolver for estimating  $b_k$  to be  $N_\epsilon \cdot \frac{1}{\Delta_k} \log(\frac{1}{\epsilon})$ . Therefore, the total number of queries to the eigensolver will be the sum of the cost of estimating each bit of  $a$ , given by

$$N_{\text{sam}}^{\text{SWAP+AE}} = \frac{1}{2\epsilon} \ln\left(\frac{1}{\epsilon}\right) \sum_{k=0}^{n-1} \frac{1}{\Delta_k} \leq \frac{\sqrt{2}}{2\epsilon} \ln\left(\frac{1}{\epsilon}\right) \log_2\left(\frac{1}{\epsilon}\right) = \frac{\sqrt{2}}{2 \ln(2)\epsilon} \ln^2\left(\frac{1}{\epsilon}\right), \quad (\text{S92})$$

where we have used the following inequalities on

$$\Delta_k \geq \Delta_{n-1} = \frac{\sqrt{2}}{2^n} b_{n-1} 2^{n-1} = \frac{1}{\sqrt{2}}, \forall k \quad (\text{S93})$$

derived from Eq. (S89) and the fact that  $b_{n-1} = 1$  from the definition of  $a = \sqrt{\frac{1+S^2}{2}}$ . This gives us

$$\sum_{k=0}^{n-1} \frac{1}{\Delta_k} \leq n \Delta_{n-1} = \sqrt{2}n = \sqrt{2} \log_2(1/\epsilon). \quad (\text{S94})$$

Note the above query complexity is independent of the amplitude  $a$  (or the overlap  $S$ ) because our estimation algorithm is constructed using fixed-point oblivious amplitude amplification.

As a comparison, in the case of only using SWAP test (no AA), the total number of samples  $N_{\text{sam}}^{\text{SWAP}}$  required to estimate  $a$  to precision  $\epsilon$  has to satisfy

$$\epsilon = \Delta a = \left| \frac{da}{dp} \right| \Delta p = \frac{1}{2} \sqrt{\frac{(1-p)}{N_{\text{sam}}^{\text{SWAP}}}}, \quad (\text{S95})$$

leading to

$$N_{\text{sam}}^{\text{SWAP}} = \left( \frac{1-S^2}{8} \right) \frac{1}{\epsilon^2} \quad (\text{S96})$$

after substituting  $p = a^2 = \frac{1+S^2}{2}$ . Comparing (S96) and (S92), we observe a quadratic speedup up to a polylog factor.

## S8. QBE ALGORITHM USING NAIVE RDM LINEAR MATCHING

In this section, for completeness, we present a QBE algorithm to perform bootstrap embedding on quantum computers by naively matching all the RDM matrix elements one by one. This scheme is inefficient as discussed in the main text due to the exponential measurement overhead. For concreteness, the algorithm as written here uses gradient descent to perform the optimization of the Lagrangian (with constraint added by Lagrange multipliers), but other gradient-based or gradient-free optimization can be used as well. We ignore the final step of tuning the global chemical potential.

---

**Algorithm 2:** Algorithm for QBE with naive linear constraint.

---

```

1 Input: Geometry of the total molecular system and the associated ab initio Hamiltonian.
2
3 /* Initialization */
4 Fragmentation: Divide the full molecular system into  $N_{frag}$  overlapping fragments;
5 for  $A = 1$  to  $N_{frag}$  do
6   Generate  $H^{(A)}$  using Eq. (S1) in Sec. S1;
7   Compute the initial full ground state density matrix:  $\rho^{(A)} \leftarrow \text{eigensolver}(H^{(A)})$ ;
8   Compute the single-qubit reduced density matrices  $\rho_r^{(A)}$  for all  $r \in O^{(A)}$ ;
9   Set  $V_{BE}^{(A)} = 0$ ;
10 Parameter initialization: Compute the initial value of the average mismatch  $\Delta\rho$ ;  $\lambda_B^{(A)} = 0$  for  $\forall A, B$ ; iter
    = 0; gd_step = 0.
11 Set the Lagrange multiplier convergence thresholds  $\epsilon_{\Delta\rho}$  and  $\epsilon_{\Delta\mu}$  to their desired initial values.
12
13 /* Main loop: */
14 while  $\Delta\rho > \epsilon_{\Delta\rho}$  do
15   for  $A = 1$  to  $N_{frag}$  do
16     Set the current learning rate  $\eta \leftarrow \text{lr\_schedule}(\text{iter})$ .
17     for gd_step = 0; gd_step ++; gd_step <  $N_{steps}$  do
18       for  $B = 1$  to  $N_{frag}$  do
19         if  $E^{(A)} \cap C^{(B)} \neq \emptyset$  then
20           Estimate the vector  $\Delta\lambda_B^{(A)}(\rho^{(A)}, \rho^{(B)})$  as defined in Eq. (16) by using  $N_{samp,0}$  (Eq. (S71))
             quantum samples to estimate each RDM element in Eq. (16).
21           Update the Lagrange multiplier vector  $\lambda_B^{(A)}$  using gradient descent:  $\lambda_B^{(A)} \leftarrow \lambda_B^{(A)} - \eta \Delta\lambda_B^{(A)}$ .
22           Generate the BE potential  $V_{BE}^{(A)}$  as defined in Eq. (17)
23           Update the Hamiltonian matrix for fragment  $A$  classical:  $H^{(A)} \leftarrow H^{(A)} + \eta V_{BE}^{(A)}$ .
24       Reduce the learning rate  $\eta$  according to  $\eta \leftarrow \eta \cdot [1 - (\text{gd\_step}/N_{steps})]$ .
25   Update the mismatch error  $\Delta\rho$  by estimating it using quantum samples.
26   for  $A = 1$  to  $N_{frag}$  do
27     Update the full ground state density matrix:  $\rho^{(A)} \leftarrow \text{eigensolver}(H^{(A)})$ ;
28     Compute the single-qubit reduced density matrices  $\rho_r^{(A)}$  for all  $r \in O^{(A)}$ ;
29   Increment iter by one: iter  $\leftarrow$  iter + 1.

```

---

In the above algorithm,  $\text{eigensolver}(H^{(A)})$  denotes the quantum eigensolver is called to find the ground state of Hamiltonian  $H^{(A)}$ . Moreover,  $\text{lr\_schedule}(\text{iter})$  is a learning rate (step size) schedule to improve convergence in gradient-descent algorithms. It returns a value for the learning rate corresponding to the **iter**-th BE iteration. One typical choice of a learning rate schedule is  $\text{lr\_schedule}(\text{iter}) \propto 1/\text{iter}$ . One crucial step of the above algorithm is to estimate the mismatch  $\Delta\rho$  as defined in Eq. (24). Here in the naive linear matching algorithm, this is accomplished by perform tomography on each RDM element as described in Sec. S6, and then classically compute the mismatch (Eq. (24)) using the estimated RDM elements.

## S9. COMPUTATIONAL DETAILS

### A. FCI and QPE Eigensolver Runtime Benchmark

Full configuration interaction (FCI) is chemists' version of exact diagonalization. In FCI, the full Hamiltonian is expanded under Slater determinant basis (i.e., *configurations*), and then a restricted Hilbert space of interest (for example, with fixed particle number and spin multiplicity) is exactly diagonalized to find the eigenstate state of interest. In the present work, we perform FCI calculation using PySCF [3] on  $H_n$  ( $n = 2, 4, 6, 8, 10, 12, 14$ ) under STO-3G basis with a fixed distance of 1 Å. The real runtime is recorded for different  $n$  and then normalized according to the runtime of  $H_2$ .

Quantum phase estimation (QPE) is a quantum algorithm to estimate the eigenstate energy and prepare the eigenstate wave function of a given Hamiltonian, whose accuracy can be systematically improved to the exact result. We give a brief overview here and refer the readers to Ref. [6] for more details on QPE including improved versions.

In QPE, the exact ground state  $|\Psi_0^A\rangle$  (or an excited state) can be prepared on a quantum computer using the quantum phase estimation algorithm followed by post-selection, given a trial state  $|\Psi_{in}^A\rangle$  is taken as the input quantum state as follows

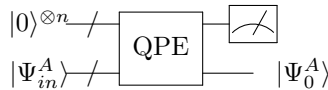

FIG. S4: Schematic for quantum phase estimation.

Analysis shows that the success probability of the post-selection process is

$$\text{Prob}[success] = |\langle \Psi_{in}^A | \Psi_0^A \rangle|^2 \left( \frac{\sin(\pi\xi)}{\pi\xi} \right)^2 \geq |\langle \Psi_{in}^A | \Psi_0^A \rangle|^2 \left( \frac{4}{\pi^2} \right), \quad (\text{S97})$$

where  $0 < \xi < \frac{1}{2}$  is the distance between the measurement outcome  $x$  (in the upper register in Fig. S4) and the true ground state energy  $\theta_0 2^n - x$ .

In the present work, for QPE runtime,  $H_n$  ( $n = 1, 2, 3, 4, 5$ ) under STO-3G basis with Jordan-Wigner mapping are used as benchmark systems. We use one evaluation qubit due to device constraint. Note the number of evaluation qubits only introduces a constant scaling factor in the absolute gate depth and will not change the scaling behavior of the QPE solver. The quantum phase estimation circuit for different hydrogen molecules is transpiled using a FAKE\_MUMBAI backend available in Qiskit [7] with a basis gate set composed of  $R_x, R_y, R_z$ , and CNOT gates. The resulting total gate depth is recorded as an estimation to the runtime of the QPE circuit. To account for the non-unity success probability of the QPE due to the finite overlap between the initial Hartree-Fock trial state and the exact ground state, the element of the CI vector corresponding to the Hartree-Fock contribution to the FCI ground state is extracted. The QPE gate depth is then rescaled by the square of the overlap amplitude. Due to the stochastic nature of the classical transpilation algorithm, the QPE circuit of each molecule is repeatedly transpiled 5 times and the smallest gate depth is used in our data. We believe this procedure results in good estimation of the real runtime of the QPE eigensolver, which includes the number of repetition required to account for the failure probability of QPE.

### B. Classical Bootstrap Embedding with VMC and FCI as Eigensolver

We implement a classical BE algorithm using variational Monte Carlo (VMC) as a stochastic eigensolver to generate the VMC data in Fig. 2 of the main text. A gradient-descent algorithm is used for the optimization. The real-space formulation of VMC with single determinant two-body Jastrow factor wavefunction as implemented in the PyQMC package [8] is used to obtain the 1-RDM of each fragment for the  $H_8$  molecule. The analytical form of the two-body Jastrow term is given in Ref. [9] which is applied to the single Slater determinants as the VMC trial wave function. The 1-RDMs of the adjacent fragments are then matched as described in Sec. 2 of the main text.

In the calculation of  $H_8$  (6 fragments in total), for each BE iteration, the VMC eigensolver is called 10 times for matching all overlapping sites. Each time the VMC is called, optimization of the Jastrow factors is first performed using roughly 10k MC samples, and then additional MC samples are accumulated in the production run to evaluate the 1-RDM. In the production run, the Monte Carlo (MC) sampling process is performed for  $N_{blocks}$  blocks. By default of PyQMC, there are 10 steps per block and 1000 configurations. We run the BE with VMC eigensolver with

three different choice of  $N_{blocks} = 4, 16, 64$ , leading to a total number of 40k, 160k, 640k MC samples in each BE iteration. We run a total of 200 BE iterations in each of the three case and plot the first 80 iterations in Fig. 2. In the case of FCI as eigensolver, we the only difference is that the 1-RDM is computed using the FCI solver, and the rest of BE iteration follows from Sec. 2. A step size of 0.05 is used for both VMC and FCI solver to perform the gradient descent based optimization in the two cases.

The density mismatch from BE with FCI and VMC eigensolver is plotted against each other. Note that since a first-quantized real space formulation of VMC is used, the VMC and FCI (second-quantized) calculation are performed in slightly different Hilbert space. This leads to different values of density mismatch from FCI and VMC in the initial BE iteration. For ease of comparison, the FCI density mismatch is rescaled by a factor of 3.8 to match the initial mismatch of the VMC.

In Fig. 2, an initial exponential convergence on the density mismatch is observed for both VMC and FCI solver. The VMC solver later plateau at a mismatch of roughly  $2 \times 10^{-3}$ , due to the statistic fluctuation on the estimated 1-RDM matrix elements from finite number of MC samples. The plateaued value of the density mismatch is calculated by taking an average of all BE iterations after iteration 30. It can be seen that as the number of MC samples increased from 40k to 640k, the fluctuations as well as the plateaued values of the density mismatch are reduced. Note since the energy is roughly quadratic in 1-RDM elements, therefore an error bar of  $2 \times 10^{-3}$  on 1-RDM elements will propagate to a reasonable accuracy (mH) on the energy.

### C. SWAP Test Circuit in Quantum Bootstrap Embedding

Two  $H_4$  molecules each with a bond length of 0.5 Å under STO-3G basis is used to generate Fig. 6 of the main text. For ease of classical simulation, the two-body terms are ignored resulting in an non-interacting Hamiltonian. An overall circuit for the SWAP estimation composed of two QPE eigensolver is given in Fig. S5 which uses 27 qubits overall. Each QPE circuit is further displayed in Fig. S6 for clarity. The resulting histogram of the QPE estimation is shown in Fig. S7, which is proportional to the probability given in Eq. (S97). The highest peak with a measurement outcome of “11011” on the 5 evaluation qubits corresponds to the many-body ground state of  $H_4$ . Post-selection is performed with this peak to ensure SWAP test is indeed estimating the overlap between the ground state. In our example, the success probability of this post-selection is roughly 0.7. Therefore, the overall post-selection success probability for two QPE solvers is  $0.7^2 \approx 0.5$ .

### D. Quantum Bootstrap Embedding Calculation

In this section, we give more computational details of the QBE calculation in infinite sampling limit as in Fig. 5 of the main text.

#### 1. QBE Iterations

For the quadratic penalty optimization, we set the penalty parameter  $\lambda = 1$  initially. In each BE iteration, the penalty parameter  $\lambda$  is increased by a factor of 25. For the linear constraint optimization, a gradient descent algorithm as described in Alg. 2 is used, where the initial step size of the gradient descent is set to 1.

#### 2. Calculation of Total System Energy

One important step after BE calculation converges is to reconstruct the total system observables. One common observable is the total system energy. In classical BE (CBE), the total system energy can be reconstructed from 1- and 2-RDM of each fragment projected to the center sites. To be concrete, the classical BE energy is defined as

$$E_{CBE} = \sum_A \sum_{p \in \mathbb{C}_A}^{N_{frag}} \left[ \sum_q^{2N_A} \left( h_{pq}^{(A)} - \frac{1}{2} G_{pq}^{(A),env} \right) P_{pq}^{(A)} + \frac{1}{2} \sum_{qrs}^{2N_A} V_{pqrs}^{(A)} \Gamma_{pqrs}^{(A)} \right], \quad (S98)$$

where  $G^{(A),env}$  is the Coulomb-exchange part of the Fock matrix in the embedding basis,  $h^{(A)}$  and  $V^{(A)}$  are the fragment 1- and 2-electron integrals,  $P^{(A)}$  and  $\Gamma^{(A)}$  are the fragment one- and two-electron reduced density matrices, respectively.

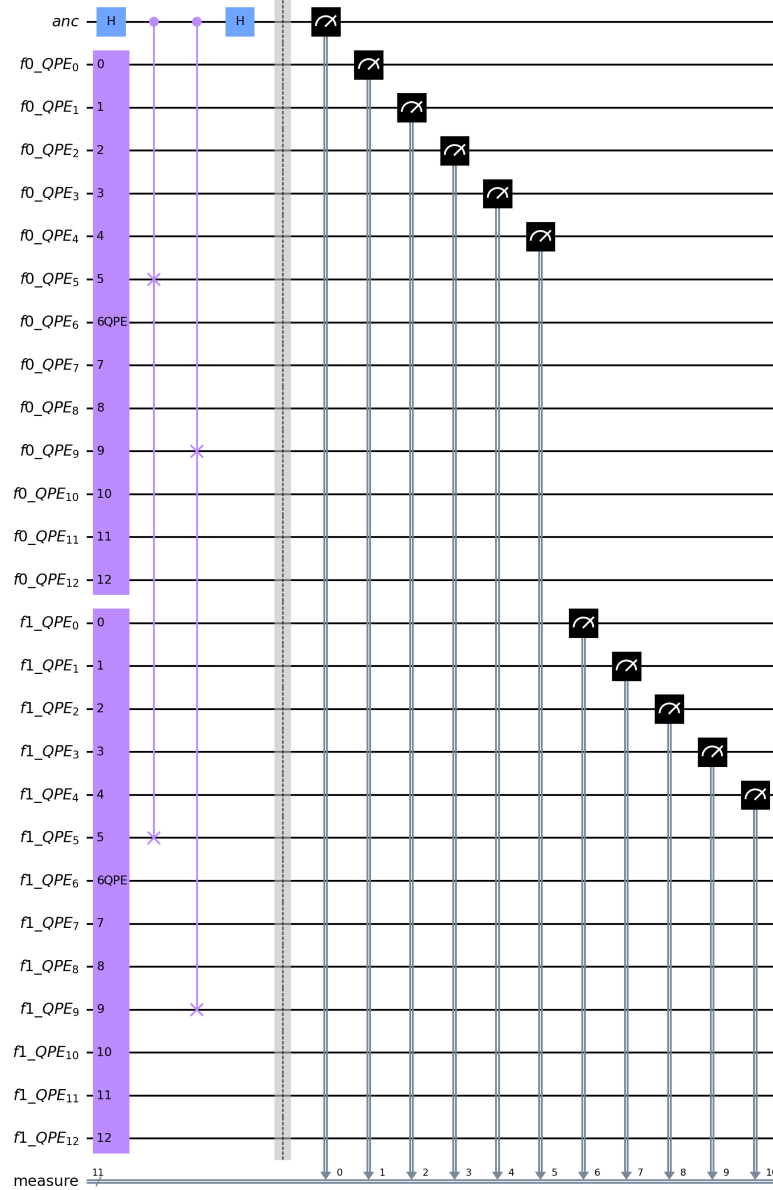

FIG. S5: SWAP test circuit between two  $H_4$  molecule with one overlapping site. Note that each QPE uses 8 system qubits and 5 evaluation qubits. The top qubit is the control ancilla for SWAP test. The overall circuit is composed of 27 qubits.

In quantum bootstrap embedding (QBE), one can certainly perform fermionic 1- and 2-RDM tomography on a quantum computer for the fragments, and then use Eq. (S98) to compute the total system energy. In our case, for simplicity, we define a similar notion of QBE energy which is used in Fig. 5 of the main text to compute the energy

$$E_{\text{QBE}} = \sum_{A=1}^{N_{\text{frag}}} \text{Tr} \left[ \rho^{(A)} H_{\text{C}}^{(A)} \right], \quad (\text{S99})$$

where  $\rho^{(A)}$  is the full density matrix of fragment  $A$ , and  $H_{\text{C}}^{(A)}$  is a projected version of  $H^{(A)}$  that involves the center site and interaction between center and the rest sites on fragment  $A$ . More concretely, we write  $H_{\text{C}}^{(A)}$  as a sum of one-

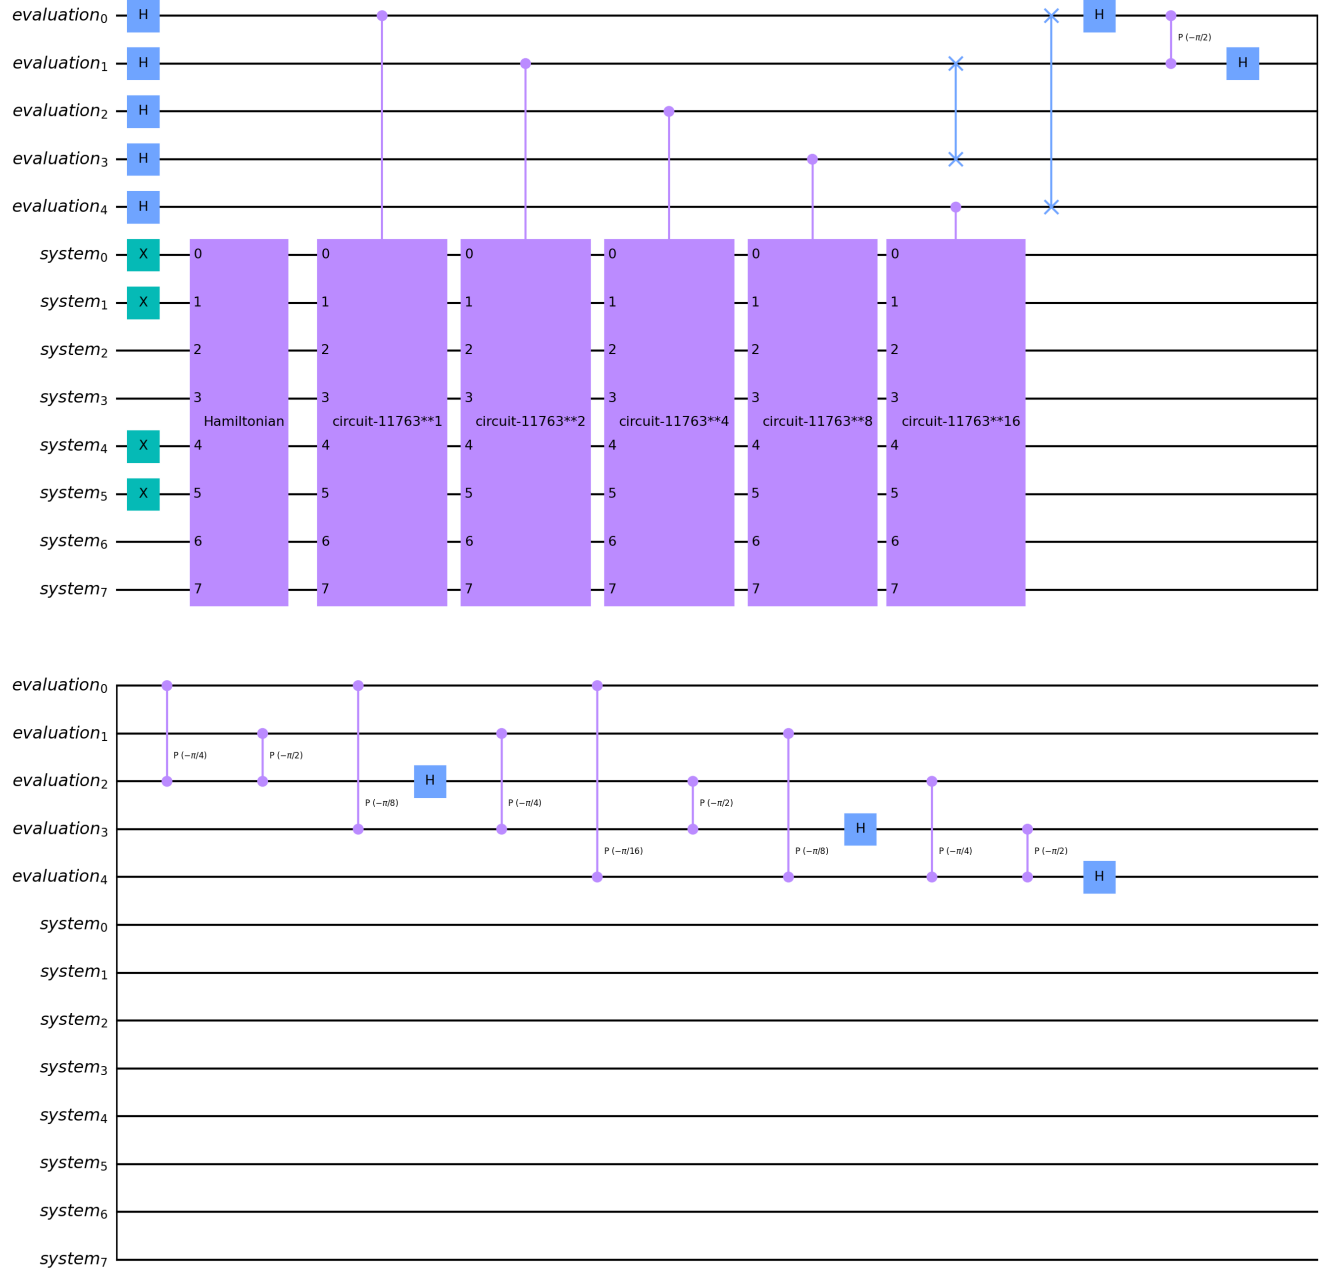

FIG. S6: A QPE circuit with for  $H_4$  molecule, where a Hartree-Fock initial trial state preparation circuit is also showed at the beginning. The circuit block labelled as “Hamiltonian” after the four initial Pauli X are a basis transformation unitary from canonical MO basis to localized orbitals (LOs).

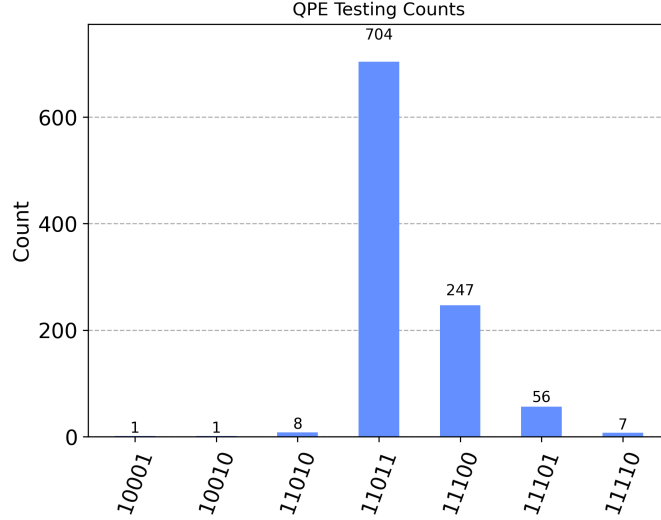

FIG. S7: Histogram of the measurement outcome of the 5 evaluation qubits for estimating the  $H_4$  ground state energy with 1024 shots. Post-selection is performed on the highest peak “11011”.

and two-body terms

$$\begin{aligned}
H_C^{(A)} &= H_{1,C}^{(A)} + H_{2,C}^{(A)}, \\
H_{1,C}^{(A)} &= \frac{1}{2} \left[ \sum_{p \in \mathbb{C}_A} \sum_q^{2N_A} h_{pq}^{(A)} + \sum_{q \in \mathbb{C}_A} \sum_p^{2N_A} h_{pq}^{(A)} \right] a_p^\dagger a_q, \\
H_{2,C}^{(A)} &= \frac{1}{8} \left[ \sum_{p \in \mathbb{C}_A} \sum_{qrs}^{2N_A} V_{pqrs}^{(A)} + \sum_{q \in \mathbb{C}_A} \sum_{prs}^{2N_A} V_{pqrs}^{(A)} + \sum_{r \in \mathbb{C}_A} \sum_{pqs}^{2N_A} V_{pqrs}^{(A)} + \sum_{s \in \mathbb{C}_A} \sum_{pqr}^{2N_A} V_{pqrs}^{(A)} \right] a_p^\dagger a_q^\dagger a_s a_r. \quad (S100)
\end{aligned}$$

Note that  $E_{\text{QBE}}$  as defined in Eq. (S100) does not exactly equal to  $E_{\text{CBE}}$  as used in classical BE calculation. There may be better ways to reconstruct  $E_{\text{CBE}}$  on a quantum computer without using fermionic density matrix tomography, and we leave this for future investigation.

### E. Details of VQE Eigensolver

In this section, we discuss how the Variational Quantum Eigensolver (VQE) can be applied as a subroutine in the Quantum Bootstrap Embedding (QBE) method for computing the ground state energy and ground state vector of different fragment Hamiltonians. Our simulations with VQE were carried out on a noiseless simulator provided in Qiskit [7].

VQE is a hybrid quantum-classical algorithm for computing the ground state (and excited states) of a Hamiltonian  $H$ , using the variation principal  $\langle \psi | H | \psi \rangle \geq E_g$  where  $|\psi\rangle$  is the normalized quantum state and  $E_g$  is the true ground state energy of  $H$ . In QBE, we may use VQE to find the ground state energy and ground state vector of the fragment Hamiltonians. Given an  $n$ -qubit fragment Hamiltonian  $H^{(A)}$  of fragment  $A$  and appropriately chosen ansatz circuit  $U_A(\theta)$  parameterized by  $\theta$ , the steps of VQE are:

1. Prepare the state  $|\psi(\theta)\rangle = U_A(\theta) |\psi_0\rangle$  on the quantum device where  $|\psi_0\rangle$  is an initial state.  $|\psi_0\rangle$  is typically chosen such that it can be prepared classically efficiently and has a non-vanishing overlap with the exact ground state of the fragment Hamiltonian (e.g., Hartree-Fock state of  $H^{(A)}$ ).
2. Measure the expectation value  $\langle \psi(\theta) | H^{(A)} | \psi(\theta) \rangle$  given a budget of  $n_{\text{shots}}$  shots (which we will specify later). We do this using the largest-degree first (LDF) algorithm [10] considering the Pauli decomposition of  $H^{(A)}$ .
3. Update ansatz parameters  $\theta$  through a classical optimizer, that will minimize the expectation value. The classical optimizer may involve computation of gradient steps or be a gradient-free method.

4. Repeat the above steps 1-3 until convergence or stopping criteria (e.g., maximum number of iterations, norm of gradient, etc.) is met.
5. Output  $|\psi(\theta)\rangle$  as the ground state vector and  $\langle\psi(\theta)|H^{(A)}|\psi(\theta)\rangle$  as the ground state energy, using the final values of the ansatz parameters  $\theta$ .

The example considered using a VQE solver in this work is a 4-qubit random spin model and a perturbed  $H_4$  linear molecule with open boundary condition under STO-3G basis. The Hamiltonian for the  $H_4$  molecule is generated first by using a H-H bond length of 1 Å (with atom labeled as 1, 2, 3, 4 from left to right). The  $H_4$  molecule is then fragmented into two fragments, where fragment  $A$  has atom 1, 2, 3 with atom 4 as a bath site. Similarly, fragment  $B$  has atom 2, 3, 4 and uses atom 1 as the bath site. Since the native  $H_4$  is too small to perform any meaningful bootstrap embedding (the two fragment already matches initially), we manually perturb atom 3 on both fragment  $A$  (right edge site) and fragment  $B$  (center site) by adding a chemical potential of +1 and -0.5, respectively.

The initial qubit Hamiltonian of each fragment is then obtained considering the Jordan-Wigner encoding. The fragment Hamiltonians are stored as set of tuples  $\{(\alpha_Q, Q)\}$  corresponding to its Pauli decomposition  $H_f = \sum_Q \alpha_Q Q$  where  $Q \in \{I, X, Y, Z\}^{\otimes n}$  is a distinct Pauli operator and  $\alpha_Q$  is the corresponding non-zero coefficient. This allows for a more compact storage rather than holding the entire matrices corresponding to the Hamiltonians in memory as there are only a polynomial in  $n$  number of non-zero coefficients  $\alpha_Q$  for each fragment Hamiltonian. Moreover, from one iteration to the next in QBE with linear constraints, this set of tuples can be efficiently updated by updating a coefficient or appending a new Pauli operator  $Q'$  along with its coefficient  $\alpha_{Q'}$  according to Eq. (17), where  $\alpha_{Q'}$  is one component of  $\lambda_B^{(A)}$ , and  $Q'$  is one-component of  $I \otimes \Sigma_r \otimes I$ .

The ansatz of each fragment in the 4-qubit random spin model is considered to be the two-local ansatz and the initial state is chosen to be  $|+\rangle^{\otimes 3}$  state. The ansatz of each fragment in the  $H_4$  chain is considered to be the UCCSD ansatz and the initial state is chosen to the Hartree-Fock state. We use the classical optimizer of the quasi-Newton method L-BFGS. The learning rate in QBE for all models is fixed to a constant value of 0.1 across iterations.

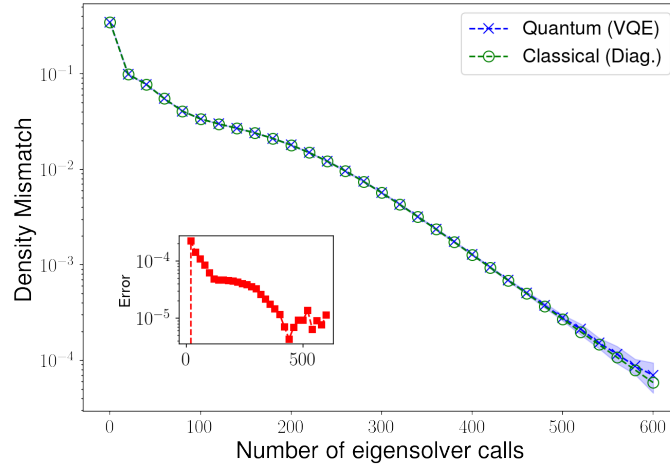

FIG. S8: Quantum bootstrap embedding convergence of the density mismatch for the 4-qubit spin model versus the number of eigenvalue calls, comparing VQE simulation (blue cross) and classical exact diagonalization (green circle). The blue shaded area shows the standard deviation from VQE estimations. The inset shows the absolute error from the VQE estimation of the mismatch to the exact value from exact diagonalization, versus number of eigenvalue calls. The number of shots considered in each step of VQE for measuring the ansatz is fixed at  $10^4$ .

Fig. S8 shows the convergence of the density mismatch for the 4-qubit spin model as the number of eigenvalue calls (note BE iteration number is roughly proportional to the number of eigensolver calls), comparing the VQE results (blue symbols) and exact classical eigensolver (green symbols). As is expected, the mismatch converges exponentially as the number of eigensolver calls increases, and the VQE results closely follow the exact results for large to intermediate density mismatch values. As the mismatch is reduced to roughly  $10^{-4}$  at about 500 eigensolver calls, the VQE results start to deviate from the exact results. The shaded area shows the uncertainty of the VQE results. The inset (red symbols) plots the deviation of the expected density mismatch (averaged over 100 independent runs) obtained from VQE with respect to the exact results, which plateaus around  $10^{-5}$ . We tentatively attribute this deviation from the exact result to the intrinsic ansatz truncation error of VQE.

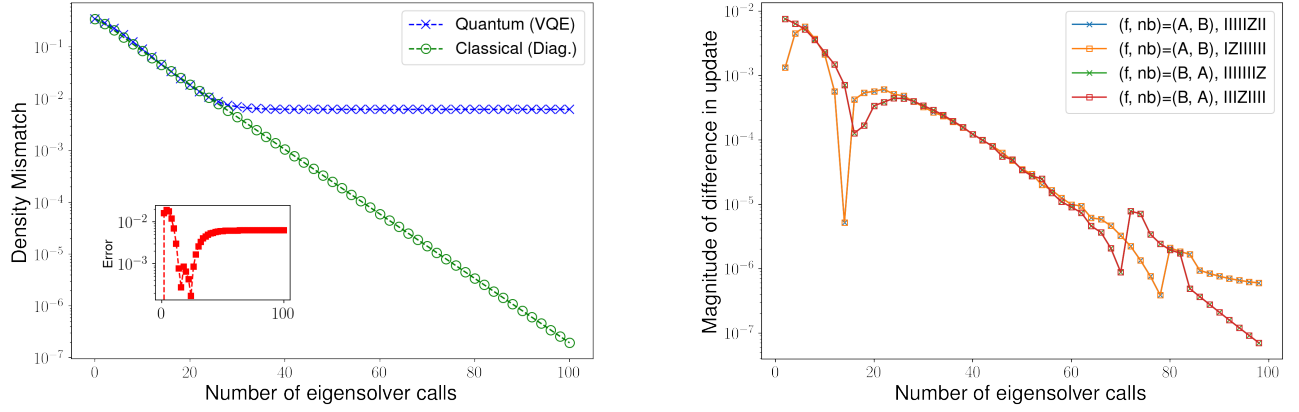

(a) Convergence behavior of density mismatch

(b) Comparison of updates in fragment Hamiltonians with QBE iterations

FIG. S9: Quantum bootstrap embedding on  $H_4$  chain. (a) We compare the convergence of the density mismatch versus the number of eigenvalue calls, comparing VQE simulation (blue cross) and classical exact diagonalization (green circle). The inset shows the absolute error from the VQE estimation of the mismatch to the exact value from exact diagonalization, versus number of eigenvalue calls. The number of shots considered in each step of VQE for measuring the ansatz is fixed at  $10^4$ . (b) We compare the difference in the magnitude of the updates of the Pauli terms (being updated or appended during QBE) in the fragment Hamiltonians between the exact solver and the VQE solver, for each pair of fragment  $f$  and neighbor  $nb$  with number of iterations. For each pair of  $(f, nb)$ , we indicate the Pauli term for each trend in the legend.

In Fig. S9(a), we show the convergence of the density mismatch on the  $H_4$  chain as a number of eigenvalue calls, comparing the VQE results (blue symbols) and exact classical eigensolver (green symbols). As observed earlier for the random spin model, the mismatch converges exponentially as the number of eigensolver calls increases, and the VQE results closely follow the exact results up to around 30 eigensolver calls. As the mismatch is reduced below  $10^{-2}$ , the VQE results start to deviate from the exact results. We tentatively attribute this deviation from the exact result to the intrinsic ansatz truncation error of VQE. To get a finer-grained understanding, in Fig S9(b), the difference in the updates between the exact solver and the VQE solver at each QBE iteration is plotted. We can see that this difference is small throughout. This difference decreases as BE iteration goes, because the absolute value of the update also decrease due to increasingly better mismatch.

- 
- [1] D. J. Thouless, *Nuclear Physics* **21**, 225 (1960).
  - [2] G. A. Quantum, Collaborators\*†, F. Arute, K. Arya, R. Babbush, D. Bacon, J. C. Bardin, R. Barends, S. Boixo, M. Broughton, B. B. Buckley, D. A. Buell, B. Burkett, N. Bushnell, Y. Chen, Z. Chen, B. Chiaro, R. Collins, W. Courtney, S. Demura, A. Dunsworth, E. Farhi, A. Fowler, B. Foxen, C. Gidney, M. Giustina, R. Graff, S. Habegger, M. P. Harrigan, A. Ho, S. Hong, T. Huang, W. J. Huggins, L. Ioffe, S. V. Isakov, E. Jeffrey, Z. Jiang, C. Jones, D. Kafri, K. Kechedzhi, J. Kelly, S. Kim, P. V. Klimov, A. Korotkov, F. Kostritsa, D. Landhuis, P. Laptev, M. Lindmark, E. Lucero, O. Martin, J. M. Martinis, J. R. McClean, M. McEwen, A. Megrant, X. Mi, M. Mohseni, W. Mruczkiewicz, J. Mutus, O. Naaman, M. Neeley, C. Neill, H. Neven, M. Y. Niu, T. E. O'Brien, E. Ostby, A. Petukhov, H. Putterman, C. Quintana, P. Roushan, N. C. Rubin, D. Sank, K. J. Satzinger, V. Smelyanskiy, D. Strain, K. J. Sung, M. Szalay, T. Y. Takeshita, A. Vainsencher, T. White, N. Wiebe, Z. J. Yao, P. Yeh, and A. Zalcman, *Science* **369**, 1084 (2020).
  - [3] Q. Sun, T. C. Berkelbach, N. S. Blunt, G. H. Booth, S. Guo, Z. Li, J. Liu, J. D. McClain, E. R. Sayfutyarova, S. Sharma, S. Wouters, and G. K.-L. Chan, *Wiley Interdisciplinary Reviews: Computational Molecular Science* **8**, e1340 (2018).
  - [4] J. M. Martyn, Z. M. Rossi, A. K. Tan, and I. L. Chuang, *PRX Quantum* **2**, 040203 (2021).
  - [5] T. J. Yoder, G. H. Low, and I. L. Chuang, *Physical Review Letters* **113**, 210501 (2014).
  - [6] K. M. Svore, M. B. Hastings, and M. Freedman, *Quantum Information and Computation* (2013).
  - [7] A. tA v, M. S. ANIS, Abby-Mitchell, H. Abraham, AduOffei, R. Agarwal, G. Agliardi, M. Aharoni, V. Ajith, I. Y. Akhalwaya, G. Aleksandrowicz, T. Alexander, M. Amy, S. Anagolum, Anthony-Gandon, I. F. Araujo, E. Arbel, A. Asfaw, I. E. Ashimine, A. Athalye, A. Avkhadiyev, C. Azaustre, P. Bhole, V. Bajpe, A. Banerjee, S. Banerjee, W. Bang, A. Bansal, P. Barkoutsos, A. Barnawal, G. Barron, G. S. Barron, L. Bello, Y. Ben-Haim, M. C. Bennett, D. Bevenius, D. Bhatnagar, P. Bhatnagar, A. Bhobe, P. Bianchini, L. S. Bishop, C. Blank, S. Bolos, S. Bopardikar, S. Bosch, S. Brandhofer, Brandon,

- S. Bravyi, Bryce-Fuller, D. Bucher, L. Burgholzer, A. Burov, F. Cabrera, P. Calpin, L. Capelluto, J. Carballo, G. Carrascal, A. Carriker, I. Carvalho, R. Chakrabarti, A. Chen, C.-F. Chen, E. Chen, J. C. Chen, R. Chen, F. Chevallier, K. Chinda, R. Cholarajan, J. M. Chow, S. Churchill, CisterMoke, C. Claus, C. Clauss, C. Clothier, R. Cocking, R. Cocuzzo, J. Connor, F. Correa, Z. Crockett, A. J. Cross, A. W. Cross, S. Cross, J. Cruz-Benito, C. Culver, A. D. Córcoles-Gonzales, N. D. S. Dague, T. E. Dandachi, A. N. Dangwal, J. Daniel, DanielAja, M. Daniels, M. Dartiaillh, A. R. Davila, F. Debouni, A. Dekusar, A. Deshmukh, M. Deshpande, D. Ding, J. Doi, E. M. Dow, P. Downing, E. Drechsler, M. S. Drudis, E. Dumitrescu, K. Dumon, I. Duran, K. EL-Safty, E. Eastman, G. Eberle, A. Ebrahimi, P. Eendebak, D. Egger, EgrettaThula, ElePT, I. Elsayed, Emilio, A. Espiricueta, M. Everitt, D. Facoetti, Farida, P. M. Fernández, S. Ferracin, D. Ferrari, A. H. Ferrera, R. Fouilland, A. Frisch, A. Fuhrer, B. Fuller, M. GEORGE, J. Gacon, B. G. Gago, C. Gambella, J. M. Gambetta, A. Gammanpila, L. Garcia, T. Garg, S. Garion, J. R. Garrison, J. Garrison, T. Gates, N. Gavrielov, G. Gentinetta, H. Georgiev, L. Gil, A. Gilliam, A. Giridharan, Glen, J. Gomez-Mosquera, Gonzalo, S. de la Puente González, J. Gorzinski, I. Gould, D. Greenberg, D. Grinko, W. Guan, D. Guijo, Guillermo-Mijares-Vilarino, J. A. Gunnels, H. Gupta, N. Gupta, J. M. Günther, M. Haglund, I. Haide, I. Hamamura, O. C. Hamido, F. Harkins, K. Hartman, A. Hasan, V. Havlicek, J. Hellmers, L. Herok, R. Hill, S. Hillmich, I. Hincks, C. Hong, H. Horii, C. Howington, S. Hu, W. Hu, C.-H. Huang, J. Huang, R. Huisman, H. Imai, T. Imamichi, K. Ishizaki, Ishwor, R. Iten, T. Itoko, A. Ivrii, A. Javadi, A. Javadi-Abhari, W. Javed, Q. Jianhua, M. Jivrajani, K. Johns, S. Johnstun, Jonathan-Shoemaker, JosDenmark, JoshDumo, J. Judge, T. Kachmann, A. Kale, N. Kanazawa, J. Kane, Kang-Bae, A. Kapila, A. Karazeev, P. Kassebaum, T. Kato, T. Kehrer, J. Kelso, S. Kelso, H. van Kemenade, V. Khanderao, S. King, Y. Kobayashi, KovillDay, A. Kovyrshin, J. Krishna, R. Krishnakumar, P. Krishnamurthy, V. Krishnan, K. Krsulich, P. Kumkar, G. Kus, LNoorl, R. LaRose, E. Lacal, R. Lambert, H. Landa, J. Lapeyre, D. Lasecki, J. Latone, S. Lawrence, C. Lee, G. Li, T. J. Liang, J. Lishman, D. Liu, P. Liu, Lolcroc, A. K. M, L. Madden, Y. Maeng, S. Maheshkar, K. Majmudar, A. Malyshev, M. E. Mandouh, J. Manela, Manjula, J. Marecek, M. Marques, K. Marwaha, D. Maslov, P. Maszota, D. Mathews, A. Matsuo, F. Mazhandu, D. McClure, M. McElaney, J. McElroy, C. McGarry, D. McKay, D. McPherson, S. Meesala, D. Meirom, C. Mendell, T. Metcalfe, M. Mevissen, A. Meyer, A. Mezzacapo, R. Midha, D. Millar, D. Miller, H. Miller, Z. Minev, A. Mitchell, A. Mohammad, N. Moll, A. Montanez, G. Monteiro, M. D. Mooring, R. Morales, N. Moran, D. Morcuende, S. Mostafa, M. Motta, R. Moynard, P. Murali, D. Murata, J. Müggenburg, T. NEMOZ, D. Nadlinger, K. Nakanishi, G. Nannicini, P. Nation, E. Navarro, Y. Naveh, S. W. Neagle, P. Neuweiler, A. Ngoueya, T. Nguyen, J. Nicander, Nick-Singstock, P. Niroula, H. Norlen, NuoWenLei, L. J. O’Riordan, O. Ogunbayo, P. Ollitrault, T. Onodera, R. Otaolea, S. Oud, D. Padilha, H. Paik, S. Pal, Y. Pang, A. Panigrahi, V. R. Pascuzzi, S. Perriello, E. Peterson, A. Phan, K. Pilch, F. Piro, M. Pistoia, C. Piveteau, J. Plewa, P. Pocreau, C. Pospel, A. Pozas-Kerstjens, R. Pracht, M. Prokop, V. Prutyantov, S. Puri, D. Puzzuoli, Pythonix, J. Pérez, Quant02, Quintiii, R. I. Rahman, A. Raja, R. Rajeev, I. Rajput, N. Ramagiri, A. Rao, R. Raymond, O. Reardon-Smith, R. M.-C. Redondo, M. Reuter, J. Rice, M. Riedemann, Rietesh, D. Risinger, P. Rivero, M. L. Rocca, D. M. Rodríguez, RohithKarur, B. Rosand, M. Rossmannek, M. Ryu, T. SAPV, N. R. C. Sa, A. Saha, A. Ash-Saki, A. Salman, S. Sanand, M. Sandberg, H. Sandesara, R. Sapra, H. Sargsyan, A. Sarkar, N. Sathaye, N. Savola, B. Schmitt, C. Schnabel, Z. Schoenfeld, T. L. Scholten, E. Schoute, J. Schuhmacher, M. Schulterbrandt, J. Schwarm, P. Schweigert, J. Seaward, Sergi, D. E. Serrano, I. F. Sertage, K. Setia, F. Shah, N. Shammah, W. Shanks, R. Sharma, P. Shaw, Y. Shi, J. Shoemaker, A. Silva, A. Simonetto, D. Singh, D. Singh, P. Singh, P. Singkanipa, Y. Siraichi, Siri, J. Sistos, J. Sistos, I. Sitdikov, S. Sivara-jah, Slavikmew, M. B. Sletfjerd, J. A. Smolin, M. Soeken, I. O. Sokolov, I. Sokolov, V. P. Soloviev, SooluThomas, Starfish, D. Steenken, M. Stypulkoski, A. Suau, S. Sun, K. J. Sung, M. Suwama, O. Słowik, R. Taeja, H. Takahashi, T. Takawale, I. Tavernelli, C. Taylor, P. Taylour, S. Thomas, K. Tian, M. Tillet, M. Tod, M. Tomasik, C. Tornow, E. de la Torre, J. L. S. Toural, K. Trabing, M. Treinish, D. Trenev, TrishaPe, F. Truger, TsafirA, G. Tsilimigkounakis, K. Tsuoka, D. Tulsi, D. Tuna, W. Turner, Y. Vaknin, C. R. Valcarce, F. Varchon, A. Vartak, A. C. Vazquez, P. Vijaywargiya, V. Villar, B. Vishnu, D. Vogt-Lee, C. Vuillot, WQ, J. Weaver, J. Weidenfeller, R. Wiczorek, J. A. Wildstrom, J. Wilson, E. Winston, WinterSoldier, J. J. Woehr, S. Woerner, R. Woo, C. J. Wood, R. Wood, S. Wood, J. Wootton, M. Wright, L. Xing, J. YU, Yaiza, B. Yang, U. Yang, J. Yao, D. Yeralin, R. Yonekura, D. Yonge-Mallo, R. Yoshida, R. Young, J. Yu, L. Yu, Yuma-Nakamura, C. Zachow, L. Zdanski, H. Zhang, E. Zheltonozhskii, I. Zidaru, B. Zimmermann, B. Zindorf, C. Zoufal, a matsuo, aeddins ibm, alexzhang13, b63, bartek bartlomiej, bcamorrison, brandhsn, nick bronn, chetmurthy, choerst ibm, comet, dalin27, deeplokhande, dekel.meirom, derwind, dime10, ehchen, ewinston, fanizzamarco, fs1132429, gadial, galeinston, georgezhou20, georgios ts, gruu, hhorii, hhyap, hykavitha, itoko, jeppevinkel, jessica angel7, jezerjojo14, jliu45, johannesgreiner, jscott2, kUmezawa, klinvill, krutik2966, ma5x, michelle4654, msuwama, nico lgrs, nrhawkins, ntgiwsvp, ordmoj, sagar pahwa, pritamsinha2304, rithikaadiga, ryancocuzzo, saktar unr, saswati qiskit, sebastian mair, septembr, sethmerkel, sg495, shaashwat, smturro2, sternparky, strickroman, tigerjack, tsura crisaldo, upsideon, vadebayo49, welien, willhbang, wmurphy collabstar, yang.luh, yuri@FreeBSD, and M. Cepulkovskis, [Qiskit: An open-source framework for quantum computing](#) (2021).
- [8] W. A. Wheeler, S. Pathak, K. Kleiner, S. Yuan, J. N. B. Rodrigues, C. Lorsche, K. Kröngchön, Y. Chang, Y. Zhou, B. Busemeyer, K. T. Williams, A. Muñoz, C. Y. Chow, and L. K. Wagner, [Pyqmc: an all-python real-space quantum monte carlo code, v0.5.1](#) (2021).
- [9] L. K. Wagner and L. Mitas, [The Journal of chemical physics](#) **126**, 034105 (2007).
- [10] D. J. Welsh and M. B. Powell, [The Computer Journal](#) **10**, 85 (1967).
