# Supplementary material for: Bootstrap Embedding on a Quantum Computer
Source: arXiv:2301.01457 source file (2023-04-25)
Supplement: Supplementary file 2 [file arxiv-help-si.tex]

\begin{filecontents}{supplement.aux}
\relax 
\providecommand\hyper@newdestlabel[2]{}
\providecommand\HyperFirstAtBeginDocument{\AtBeginDocument}
\HyperFirstAtBeginDocument{\ifx\hyper@anchor\@undefined
\global\let\oldnewlabel\newlabel
\gdef\newlabel#1#2{\newlabelxx{#1}#2}
\gdef\newlabelxx#1#2#3#4#5#6{\oldnewlabel{#1}{{#2}{#3}}}
\AtEndDocument{\ifx\hyper@anchor\@undefined
\let\newlabel\oldnewlabel
\fi}
\fi}
\global\let\hyper@last\relax 
\gdef\HyperFirstAtBeginDocument#1{#1}
\providecommand\HyField@AuxAddToFields[1]{}
\providecommand\HyField@AuxAddToCoFields[2]{}
\gdef \tocmax@section{17.83337pt}
\gdef \tocmax@subsection{14.91669pt}
\gdef \tocmax@subsubsection{12.2778pt}
\gdef \tocmax@paragraph{5.0pt}
\gdef \tocmax@appendix{5.0pt}
\gdef \tocmax@pagenum{10.00003pt}
\providecommand \oddpage@label [2]{}
\newlabel{FirstPage}{{}{1}{}{Doc-Start}{}}
\@writefile{toc}{\contentsline {title}{Supporting Information for ``Bootstrap Embedding on a Quantum Computer"}{1}{section*.1}\protected@file@percent }
\@writefile{toc}{\tocdepth@munge}
\@writefile{toc}{\contentsline {section}{\numberline {}Contents}{1}{section*.2}\protected@file@percent }
\@writefile{toc}{\tocdepth@restore}
\citation{thouless1960stability}
\citation{google2020hartree}
\citation{thouless1960stability}
\@writefile{toc}{\contentsline {section}{\numberline {S1}Construction of the Embedding Hamiltonians}{2}{section*.3}\protected@file@percent }
\newlabel{app:frag}{{S1}{2}{}{section*.3}{}}
\newlabel{embedding-projection-int}{{S1}{2}{}{equation.1.1}{}}
\@writefile{toc}{\contentsline {section}{\numberline {S2}Basis Transformation Unitary from Localized to Canonical Molecular Orbitals}{2}{section*.4}\protected@file@percent }
\newlabel{app:lo-mo-basis-trans-unitary}{{S2}{2}{}{section*.4}{}}
\citation{sun2018pyscf}
\@writefile{toc}{\contentsline {section}{\numberline {S3}Proof of Equivalence of the Linear and Quadratic Constraint}{3}{section*.5}\protected@file@percent }
\newlabel{app:constraint-equivalent-proof}{{S3}{3}{}{section*.5}{}}
\newlabel{app:rdm-def}{{S11}{3}{}{equation.3.11}{}}
\newlabel{quadratic-decompose}{{S12}{3}{}{equation.3.12}{}}
\newlabel{orthonormal-sigmas}{{S17}{3}{}{equation.3.17}{}}
\newlabel{dl-dlambda-sum-rep}{{S18}{4}{}{equation.3.18}{}}
\@writefile{toc}{\contentsline {section}{\numberline {S4}Estimating Quadratic Penalty from Subsystem $\mathtt  {SWAP}$ Test}{4}{section*.6}\protected@file@percent }
\newlabel{app:swap-test}{{S4}{4}{}{section*.6}{}}
\@writefile{toc}{\contentsline {subsection}{\numberline {A}Quantum Circuit of the $\mathtt  {SWAP}$ Test}{4}{section*.7}\protected@file@percent }
\@writefile{lof}{\contentsline {figure}{\numberline {S1}{\ignorespaces Subsystem $\mathtt  {SWAP}$ test between the overlapping regions of fragment $A$ and $B$, where a controlled $\mathtt  {SWAP}$ operation is performed on $A_0$ and $B_0$. The measurement probability of the top ancilla qubit encodes information of the overlap.\relax }}{4}{figure.caption.8}\protected@file@percent }
\providecommand*\caption@xref[2]{\@setref\relax\@undefined{#1}}
\newlabel{sfig:sub-swap}{{S1}{4}{Subsystem $\mathtt {SWAP}$ test between the overlapping regions of fragment $A$ and $B$, where a controlled $\mathtt {SWAP}$ operation is performed on $A_0$ and $B_0$. The measurement probability of the top ancilla qubit encodes information of the overlap.\relax }{figure.caption.8}{}}
\@writefile{toc}{\contentsline {subsection}{\numberline {B}Ancilla Measurement Probability}{4}{section*.9}\protected@file@percent }
\newlabel{psiA}{{S20}{5}{}{equation.4.20}{}}
\newlabel{psiB}{{S21}{5}{}{equation.4.21}{}}
\newlabel{probm0}{{S22}{5}{}{equation.4.22}{}}
\newlabel{cross-overlap}{{S25}{5}{}{equation.4.25}{}}
\newlabel{from-swap-prob-to-overlap}{{S26}{5}{}{equation.4.26}{}}
\newlabel{self-overlap}{{S27}{6}{}{equation.4.27}{}}
\@writefile{toc}{\contentsline {subsection}{\numberline {C}Connection to Quadratic Penalty}{6}{section*.10}\protected@file@percent }
\@writefile{toc}{\contentsline {section}{\numberline {S5}Eigenvalue Equations for the Quadratic Penalty Method}{6}{section*.11}\protected@file@percent }
\newlabel{app:gradient-quadratic}{{S5}{6}{}{section*.11}{}}
\newlabel{deltaL=0}{{S30}{6}{}{equation.5.30}{}}
\@writefile{toc}{\contentsline {subsection}{\numberline {A}Derivative $\frac  {\partial \mathcal  {L}_A}{\partial C_{ai\mu }}$}{7}{section*.12}\protected@file@percent }
\newlabel{app:dldc}{{S5\,A}{7}{}{section*.12}{}}
\newlabel{1st-deriv-phiA}{{S45}{8}{}{equation.5.45}{}}
\newlabel{dLdC*}{{S49}{8}{}{equation.5.49}{}}
\@writefile{toc}{\contentsline {subsection}{\numberline {B}Derivative $\frac  {\partial C_{ai\mu }}{\delta V_{\rm  BE}}$}{8}{section*.13}\protected@file@percent }
\newlabel{app:dcdv}{{S5\,B}{8}{}{section*.13}{}}
\newlabel{1st-perturb-wf}{{S51}{9}{}{equation.5.51}{}}
\newlabel{1st-perturb-wf-expand}{{S53}{9}{}{equation.5.53}{}}
\newlabel{1st-perturb-coeff}{{S54}{9}{}{equation.5.54}{}}
\newlabel{1st-perturb-coeff-final}{{S58}{9}{}{equation.5.58}{}}
\@writefile{toc}{\contentsline {subsection}{\numberline {C}Gradient of Cost Function versus BE Potential}{10}{section*.14}\protected@file@percent }
\newlabel{app:together}{{S5\,C}{10}{}{section*.14}{}}
\newlabel{final-dldv}{{S62}{10}{}{equation.5.62}{}}
\@writefile{toc}{\contentsline {section}{\numberline {S6}Sample Complexity for Estimating the Overlap from Tomography}{10}{section*.15}\protected@file@percent }
\newlabel{app:sample-advantage-lin-quad}{{S6}{10}{}{section*.15}{}}
\newlabel{s2-as-rdm-element}{{S63}{10}{}{equation.6.63}{}}
\newlabel{var-S2}{{S67}{11}{}{equation.6.67}{}}
\newlabel{seq:tmg-per-element}{{S71}{11}{}{equation.6.71}{}}
\citation{martyn2021grand_si}
\citation{yoder2014fixed_si}
\@writefile{toc}{\contentsline {section}{\numberline {S7}Details of Quantum Amplitude Estimation and Quadratic Speedup}{12}{section*.16}\protected@file@percent }
\newlabel{app:aa+binary-search}{{S7}{12}{}{section*.16}{}}
\@writefile{toc}{\contentsline {subsection}{\numberline {A}Amplitude Amplification}{12}{section*.17}\protected@file@percent }
\newlabel{app:amplitude-amp}{{S7\,A}{12}{}{section*.17}{}}
\newlabel{amp-amp}{{S73}{12}{}{equation.7.73}{}}
\newlabel{state-A0}{{S74}{12}{}{equation.7.74}{}}
\newlabel{state-B0}{{S75}{12}{}{equation.7.75}{}}
\newlabel{amp-overlap}{{S77}{12}{}{equation.7.77}{}}
\newlabel{Aperp}{{S78}{12}{}{equation.7.78}{}}
\citation{martyn2021grand_si}
\@writefile{lof}{\contentsline {figure}{\numberline {S2}{\ignorespaces Quantum circuit to estimate the ground state overlap between subsystems of two fragments, composed of two quantum eigensolver (QES) for two fragments ground state wave function followed by a $\mathtt  {SWAP}$ test. The circuit in the dashed box is $U$ in Eq. \eqref  {amp-amp} which will be repeated multiple times during the amplitude amplification process as will be discussed in the following.\relax }}{13}{figure.caption.18}\protected@file@percent }
\newlabel{sfig:U_prep}{{S2}{13}{Quantum circuit to estimate the ground state overlap between subsystems of two fragments, composed of two quantum eigensolver (QES) for two fragments ground state wave function followed by a $\swap $ test. The circuit in the dashed box is $U$ in Eq. \eqref {amp-amp} which will be repeated multiple times during the amplitude amplification process as will be discussed in the following.\relax }{figure.caption.18}{}}
\newlabel{Bphi}{{S83}{13}{}{equation.7.83}{}}
\citation{martyn2021grand_si}
\newlabel{Aphi}{{S86}{14}{}{equation.7.86}{}}
\@writefile{lof}{\contentsline {figure}{\numberline {S3}{\ignorespaces Quantum circuit for fixed-point oblivious amplitude amplification of the coherent quantum matching. The quantum gates in dashed box corresponds to the gates in bracket of Eq. \eqref  {amp-amp} which needs to be repeated by $d/2$ times, where $d$ will be determined by the slope of the amplification polynomial $\frac  {1}{\Delta _k}$ (more about this in the next section).\relax }}{14}{figure.caption.19}\protected@file@percent }
\newlabel{sfig:swap-aa}{{S3}{14}{Quantum circuit for fixed-point oblivious amplitude amplification of the coherent quantum matching. The quantum gates in dashed box corresponds to the gates in bracket of Eq. \eqref {amp-amp} which needs to be repeated by $d/2$ times, where $d$ will be determined by the slope of the amplification polynomial $\frac {1}{\Delta _k}$ (more about this in the next section).\relax }{figure.caption.19}{}}
\@writefile{toc}{\contentsline {subsection}{\numberline {B}Estimate the Amplitude from Binary Search}{14}{section*.20}\protected@file@percent }
\newlabel{app:binary-search}{{S7\,B}{14}{}{section*.20}{}}
\newlabel{aeq:Deltak}{{S89}{14}{}{equation.7.89}{}}
\newlabel{n_eps}{{S91}{15}{}{equation.7.91}{}}
\@writefile{toc}{\contentsline {subsection}{\numberline {C}Quadratic Speedup}{15}{section*.21}\protected@file@percent }
\newlabel{app:quadratic-speedup}{{S7\,C}{15}{}{section*.21}{}}
\newlabel{n_samp_swap+ae}{{S92}{15}{}{equation.7.92}{}}
\newlabel{n_samp_swap}{{S96}{15}{}{equation.7.96}{}}
\citation{sun2018pyscf}
\@writefile{toc}{\contentsline {section}{\numberline {S8}QBE Algorithm Using Naive RDM Linear Matching}{16}{section*.22}\protected@file@percent }
\newlabel{app:linear-alg}{{S8}{16}{}{section*.22}{}}
\@writefile{loa}{\contentsline {algocf}{\numberline {2}{\ignorespaces Algorithm for QBE with naive linear constraint.\relax }}{16}{algocf.2}\protected@file@percent }
\newlabel{alg:qbe_linearcons}{{2}{16}{}{algocf.2}{}}
\citation{svore2013faster_si}
\citation{Qiskit}
\citation{wheeler2021pyqmc}
\@writefile{toc}{\contentsline {section}{\numberline {S9}Computational Details}{17}{section*.23}\protected@file@percent }
\newlabel{app:computational-details}{{S9}{17}{}{section*.23}{}}
\@writefile{toc}{\contentsline {subsection}{\numberline {A}FCI and QPE Eigensolver Runtime Benchmark}{17}{section*.24}\protected@file@percent }
\@writefile{lof}{\contentsline {figure}{\numberline {S4}{\ignorespaces Schematic for quantum phase estimation.\relax }}{17}{figure.caption.25}\protected@file@percent }
\newlabel{fig:qpe}{{S4}{17}{Schematic for quantum phase estimation.\relax }{figure.caption.25}{}}
\newlabel{qpe_suc_prob}{{S97}{17}{}{equation.9.97}{}}
\@writefile{toc}{\contentsline {subsection}{\numberline {B}Classical Bootstrap Embedding with VMC and FCI as Eigensolver}{17}{section*.26}\protected@file@percent }
\newlabel{app:be-vmc}{{S9\,B}{17}{}{section*.26}{}}
\@writefile{toc}{\contentsline {subsection}{\numberline {C}$\mathtt  {SWAP}$ Test Circuit in Quantum Bootstrap Embedding}{18}{section*.27}\protected@file@percent }
\newlabel{app:swap-test-circuit}{{S9\,C}{18}{}{section*.27}{}}
\@writefile{toc}{\contentsline {subsection}{\numberline {D}Quantum Bootstrap Embedding Calculation}{18}{section*.31}\protected@file@percent }
\newlabel{app:qbe-calculation}{{S9\,D}{18}{}{section*.31}{}}
\@writefile{toc}{\contentsline {subsubsection}{\numberline {1}QBE Iterations}{18}{section*.32}\protected@file@percent }
\@writefile{toc}{\contentsline {subsubsection}{\numberline {2}Calculation of Total System Energy}{18}{section*.33}\protected@file@percent }
\newlabel{app:energy-calc}{{S9\,D\,2}{18}{}{section*.33}{}}
\newlabel{cbe-energy-def}{{S98}{18}{}{equation.9.98}{}}
\@writefile{lof}{\contentsline {figure}{\numberline {S5}{\ignorespaces $\mathtt  {SWAP}$ test circuit between two H$_4$ molecule with one overlapping site. Note that each QPE uses 8 system qubits and 5 evaluation qubits. The top qubit is the control ancilla for $\mathtt  {SWAP}$ test. The overall circuit is composed of 27 qubits.\relax }}{19}{figure.caption.28}\protected@file@percent }
\newlabel{sfig:swap}{{S5}{19}{$\swap $ test circuit between two H$_4$ molecule with one overlapping site. Note that each QPE uses 8 system qubits and 5 evaluation qubits. The top qubit is the control ancilla for $\swap $ test. The overall circuit is composed of 27 qubits.\relax }{figure.caption.28}{}}
\@writefile{lof}{\contentsline {figure}{\numberline {S6}{\ignorespaces A QPE circuit with for H$_4$ molecule, where a Hartree-Fock initial trial state preparation circuit is also showed at the beginning. The circuit block labelled as ``Hamiltonian" after the four initial Pauli X are a basis transformation unitary from canonical MO basis to localized orbitals (LOs).\relax }}{20}{figure.caption.29}\protected@file@percent }
\newlabel{sfig:qpe-h4}{{S6}{20}{A QPE circuit with for H$_4$ molecule, where a Hartree-Fock initial trial state preparation circuit is also showed at the beginning. The circuit block labelled as ``Hamiltonian" after the four initial Pauli X are a basis transformation unitary from canonical MO basis to localized orbitals (LOs).\relax }{figure.caption.29}{}}
\citation{Qiskit}
\citation{welsh1967upper}
\@writefile{lof}{\contentsline {figure}{\numberline {S7}{\ignorespaces Histogram of the measurement outcome of the 5 evaluation qubits for estimating the H$_4$ ground state energy with 1024 shots. Post-selection is performed on the highest peak ``11011".\relax }}{21}{figure.caption.30}\protected@file@percent }
\newlabel{sfig:qpe-h4-count}{{S7}{21}{Histogram of the measurement outcome of the 5 evaluation qubits for estimating the H$_4$ ground state energy with 1024 shots. Post-selection is performed on the highest peak ``11011".\relax }{figure.caption.30}{}}
\newlabel{qbe-energy-def}{{S100}{21}{}{equation.9.100}{}}
\@writefile{toc}{\contentsline {subsection}{\numberline {E}Details of VQE Eigensolver}{21}{section*.34}\protected@file@percent }
\newlabel{app:vqe}{{S9\,E}{21}{}{section*.34}{}}
\@writefile{lof}{\contentsline {figure}{\numberline {S8}{\ignorespaces Quantum bootstrap embedding convergence of the density mismatch for the 4-qubit spin model versus the number of eigenvalue calls, comparing VQE simulation (blue cross) and classical exact diagonalization (green circle). The blue shaded area shows the standard deviation from VQE estimations. The inset shows the absolute error from the VQE estimation of the mismatch to the exact value from exact diagonalization, versus number of eigenvalue calls. The number of shots considered in each step of VQE for measuring the ansatz is fixed at $10^{4}$.\relax }}{22}{figure.caption.35}\protected@file@percent }
\newlabel{sfig:spin-model-vqe}{{S8}{22}{Quantum bootstrap embedding convergence of the density mismatch for the 4-qubit spin model versus the number of eigenvalue calls, comparing VQE simulation (blue cross) and classical exact diagonalization (green circle). The blue shaded area shows the standard deviation from VQE estimations. The inset shows the absolute error from the VQE estimation of the mismatch to the exact value from exact diagonalization, versus number of eigenvalue calls. The number of shots considered in each step of VQE for measuring the ansatz is fixed at $10^{4}$.\relax }{figure.caption.35}{}}
\bibdata{supplementNotes,ref}
\bibcite{thouless1960stability}{{1}{1960}{{Thouless}}{{}}}
\bibcite{google2020hartree}{{2}{2020}{{Quantum\ \emph  {et~al.}}}{{Quantum, Collaborators*†, Arute, Arya, Babbush, Bacon, Bardin, Barends, Boixo, Broughton, Buckley \emph  {et~al.}}}}
\bibcite{sun2018pyscf}{{3}{2018}{{Sun\ \emph  {et~al.}}}{{Sun, Berkelbach, Blunt, Booth, Guo, Li, Liu, McClain, Sayfutyarova, Sharma \emph  {et~al.}}}}
\bibcite{martyn2021grand_si}{{4}{2021}{{Martyn\ \emph  {et~al.}}}{{Martyn, Rossi, Tan,\ and\ Chuang}}}
\bibcite{yoder2014fixed_si}{{5}{2014}{{Yoder\ \emph  {et~al.}}}{{Yoder, Low,\ and\ Chuang}}}
\bibcite{svore2013faster_si}{{6}{2013}{{Svore\ \emph  {et~al.}}}{{Svore, Hastings,\ and\ Freedman}}}
\bibcite{Qiskit}{{7}{2021}{{tA~v\ \emph  {et~al.}}}{{tA~v, ANIS, Abby-Mitchell, Abraham, AduOffei \emph  {et~al.}}}}
\bibcite{wheeler2021pyqmc}{{8}{2021}{{Wheeler\ \emph  {et~al.}}}{{Wheeler, Pathak, Rodrigues, Lorsung, Chang, Zhou, Busemeyer, Williams, Munoz, Wagner \emph  {et~al.}}}}
\bibcite{welsh1967upper}{{9}{1967}{{Welsh\ and\ Powell}}{{}}}
\bibstyle{apsrev4-2}
\@writefile{lof}{\contentsline {figure}{\numberline {S9}{\ignorespaces Quantum bootstrap embedding on H$_4$ chain. (a) We compare the convergence of the density mismatch versus the number of eigenvalue calls, comparing VQE simulation (blue cross) and classical exact diagonalization (green circle). The inset shows the absolute error from the VQE estimation of the mismatch to the exact value from exact diagonalization, versus number of eigenvalue calls. The number of shots considered in each step of VQE for measuring the ansatz is fixed at $10^{4}$. (b) We compare the difference in the magnitude of the updates of the Pauli terms (being updated or appended during QBE) in the fragment Hamiltonians between the exact solver and the VQE solver, for each pair of fragment $f$ and neighbor $nb$ with number of iterations. For each pair of $(f,nb)$, we indicate the Pauli term for each trend in the legend. \relax }}{23}{figure.caption.36}\protected@file@percent }
\newlabel{sfig:H4_qbe_vqe}{{S9}{23}{Quantum bootstrap embedding on H$_4$ chain. (a) We compare the convergence of the density mismatch versus the number of eigenvalue calls, comparing VQE simulation (blue cross) and classical exact diagonalization (green circle). The inset shows the absolute error from the VQE estimation of the mismatch to the exact value from exact diagonalization, versus number of eigenvalue calls. The number of shots considered in each step of VQE for measuring the ansatz is fixed at $10^{4}$. (b) We compare the difference in the magnitude of the updates of the Pauli terms (being updated or appended during QBE) in the fragment Hamiltonians between the exact solver and the VQE solver, for each pair of fragment $f$ and neighbor $nb$ with number of iterations. For each pair of $(f,nb)$, we indicate the Pauli term for each trend in the legend. \relax }{figure.caption.36}{}}
\@writefile{toc}{\contentsline {section}{\numberline {}References}{23}{section*.37}\protected@file@percent }
\newlabel{LastBibItem}{{9}{23}{}{section*.37}{}}
\newlabel{LastPage}{{}{23}{}{}{}}
\gdef \@abspage@last{23}
\end{filecontents}
